# Supplementary material for: Dynamic Matching with Post-allocation Service and its Application to Refugee Resettlement
Source: arXiv:2410.22992 source file (2025-07-02)
Supplement: Supplementary file 1 [file apx+ALG+P+motivation.tex]

\subsection{Motivating Numerical Example for \CO{} (\texorpdfstring{\Cref{ALG+Surrogate+P}}{})}\label{apx+ALG+P+motivation}
\SLcomment{This appendix needs to be removed}

To further motivate our rationale behind the development of \Cref{ALG+Surrogate+P}, we illustrate its potential as a viable complement to \Cref{ALG+Surrogate+D} through a numerical example. Consider a scenario where the agency lacks access to accurate information about the backlogs.
However, the agency has imperfect knowledge of service rates. In this situation, the agency can simulate the backlog dynamics for each affiliate using its (imperfect) knowledge of the service rates. In the following example, we demonstrate the limitation of such an approach.

Concretely, consider a numerical example with a single affiliate ($m=1$), $\TotalTime=1000$ arrivals with no tied cases, and rewards following a uniform distribution on the interval $(0,1)$. The capacity ratio is set at $\CapRatio=0.5$, and the \emph{actual} service rate is $\ServiceRate = 0.51$ (i.e., $\ServiceSlack=0.01$). However, assume that the agency lacks knowledge of both the actual \backlog{} process and the precise service rate. Instead, it simulates the \backlog{} process based on a mis-specified service rate of $\hat{\ServiceRate} =0.6$.

In the table \ref{tab:algorithm_performance}, we present the performance of (i) \Cref{ALG+Surrogate+D} under full knowledge of the actual \backlog{}, (ii) \Cref{ALG+Surrogate+D} operated under simulated \backlog{} with the mis-specified service rate $\hat{\ServiceRate}=0.6$, and (iii) \Cref{ALG+Surrogate+P} (which operates without requiring any knowledge of the \backlog{} or service rate). The objective value is computed based on $\BuildUpCost = 10$.
\begin{table}[h]
\centering
\begin{tabular}{lccc}
\hline
\textbf{Algorithm} & \textbf{Reward} & \textbf{Average \backlog{}} & \textbf{Objective ($\BuildUpCost=10$)} \\
\hline
\Cref{ALG+Surrogate+D} with knowledge of \backlog{} & 350.42 & 1.57 & 334.72 \\
\Cref{ALG+Surrogate+D} with mis-specified service rate & 363.62 & 7.38 & 289.82 \\
\Cref{ALG+Surrogate+P} & 365.19 & 6.58 & 299.39 \\
\hline
\end{tabular}
\caption{Numerical illustration: performance of \Cref{ALG+Surrogate+D} (with and without correct knowledge of \backlog{}s) and \Cref{ALG+Surrogate+P} (note: we set $\boldsymbol{\eta=\zeta =5/\sqrt{\TotalTime}}$ for \Cref{ALG+Surrogate+D} and $\boldsymbol{\eta_\Timeidx = 5/\sqrt{\Timeidx}}$ for \Cref{ALG+Surrogate+P}. The result is based on averaging over 1000 sample paths of arrivals and services.)}
\label{tab:algorithm_performance}
\end{table}
We observe that, while \Cref{ALG+Surrogate+D} with the correct \backlog{} outperforms \Cref{ALG+Surrogate+P} in terms of the objective value. However, if \Cref{ALG+Surrogate+D} uses the simulated backlog information with the mis-specified service rates, its performance degrades. Specifically, \Cref{ALG+Surrogate+D} with the mis-specified service rate shows a higher average \backlog{} and a lower reward than \Cref{ALG+Surrogate+P}.
