# Supplementary material for: Dynamic Matching with Post-allocation Service and its Application to Refugee Resettlement
Source: arXiv:2410.22992 source file (2025-07-02)
Supplement: Supplementary file 2 [file apx+ALG+P+stop+complete.tex]

\subsubsection{Missing Details for Proofs in Appendix \ref{apx+B-2}}\label{apx+ALG+P+stop}\hfill\\
%%%%%%%%%%%%%%%%% texts %%%%%%%%%%%%%%%
In this subsection, we explain how to make the arguments made in Appendix \ref{apx+B-2} more precise. In particular, in the proof of Claim \ref{claim:A} (Appendix \ref{apx+B-2}), we assumed that the optimization problem \eqref{line:const} is always feasible for the sake of simplicity.\footnote{Note that this is always true in the absence of tied cases.} Let $\mathcal{G}_\Timeidx$ be the event that that the \eqref{line:const} admits a feasible solution. Here we show that incorporating the precise high-probability bound of $\mathcal{G}_\Timeidx$ does not affect our main result (i.e., \Cref{claim:stop+bound+P} and \Cref{lemma:B-2}).\par 
We first begin by incorporating the probability of $\mathcal{G}_\Timeidx$ to the proof of \Cref{apx+B-2}. The only part we need to modify is Claim \ref{claim:A}. Let $N_{\Timeidx, \Locidx}$ be the total number of tied cases at affiliate $\Locidx$ up to time $\Timeidx$. We first note that the program \eqref{line:const} admits a feasible solution if and only if $N_{\Timeidx, \Locidx} \leq \CapRatio_\Locidx \Timeidx$ for all $\Locidx \in [\Locnum]$. 
We further recall that we assumed that $\P[\Target_\Timeidx = \Locidx] = \CapRatio_\Locidx - d_i$ for some positive constant $d_i>0$. Hence, by Azuma-Hoeffding inequality and the union bound, we have:
\begin{equation}
\P[\mathcal{G}_\Timeidx] \geq 1 -\sum_{\Locidx=1}^\Locnum \exp\left(-\frac{d_i^2 \Timeidx}{2}\right) := 1 - g(t)
\end{equation}
where in the last line we define $g(t) := \sum_{\Locidx=1}^\Locnum \exp\left(-\frac{d_i^2 \Timeidx}{2}\right)$. Incorporating the above high-probability bound, the precise statement of Claim \ref{claim:A} becomes the following:
\begin{claim}
There exists constant $M_{\textsf{A}}$ such that, for any given $\delta \in (0,1)$, the term $\textsf{(A)}$ in line \eqref{line:lemma+over} satisfies:
\begin{equation*}
\textsf{(A)}\leq 
%\SLedit{
\sum_{\Locidx=1}^\Locnum \nu^*_{\Timeidx, i}\left(
 \sum_{\Tauidx=1}^\Timeidx \Decision_{\Tauidx, \Locidx}^{\textsf{(M)}} - \Timeidx\CapRatio_\Locidx 
\right)
%} 
+ M_{\textsf{A}}\sqrt{t\log(1/\delta)}
\end{equation*}
with probability at least 
%\SLedit{
$1-\delta - g(t)$
%} 
and for some $0 \leq  \nu^*_{\Timeidx, i} \leq 1$.
\end{claim}

The rest of the proofs in \Cref{apx+B-2} does not change. Hence, the statement of \Cref{lemma:goal} now changes to
\begin{lemma}\label{lemma:Z+precise}
For any fixed $\Timeidx$, there exists a constant $a>0$ for which 
\begin{equation*}
\P\left[\mathbf{Z}_\Timeidx^{\textsf{(M)}} \leq t\CapRatioVec + a\sqrt{t\log(1/\delta)}\mathbf{1}\right] \geq 
%\SLedit{
1-\delta -g(t)
%} 
\end{equation*}
where $\textbf{1}$ is the vector of ones.
\end{lemma}

By following the same steps from lines \eqref{line:def+T+delta} to \eqref{line:line:def+T+delta+end} with \Cref{lemma:Z+precise}, the statement of Proposition \Cref{claim:stop+bound+P} accordingly changes to the following.
\begin{proposition}\label{prop+stop+precise}
For \CO{} (\Cref{ALG+Surrogate+P}), for any given $\delta \in (0,1)$, we have
\begin{equation*}
\TotalTime - \StoppingMod \leq  \frac{a}{\underline{\CapRatio}}\sqrt{\TotalTime\log(1/\delta)} + \frac{1}{\underline{\CapRatio}}
\end{equation*}
with probability at least 
%\SLedit{
$1-\delta - g(T(\delta))$
%}
where constant $a>0$ is given by \Cref{lemma:Z+precise} and $T(\delta) := T - \frac{a}{\underline{\rho}}\sqrt{\TotalTime\log(1/\delta)} - \frac{1}{\underline{\rho}}$.
\end{proposition}

Finally, we show that \Cref{prop+stop+precise} implies $\BigO(\TotalTime)$ upper bound on $\E[(\TotalTime - \StoppingMod)^2]$, as we desired for \Cref{lemma:B-2}. It suffices to show $\E[(\TotalTime - \StoppingMod - \frac{1}{\underline{\CapRatio}})] \leq \BigO(\TotalTime)$.\footnote{
To see this, we note that
$\E[(\TotalTime - \StoppingMod )^2]$ = 
$\E[(\TotalTime - \StoppingMod - \frac{1}{\underline{\CapRatio}} + \frac{1}{\underline{\CapRatio}})^2] =
\E[(\TotalTime - \StoppingMod - \frac{1}{\underline{\CapRatio}})^2] + \frac{2}{\underline{\CapRatio}}\E[T-\StoppingMod] + \frac{1}{\underline{\CapRatio}^2} \leq \E[(\TotalTime - \StoppingMod - \frac{1}{\underline{\CapRatio}} )^2] + \BigO(\TotalTime)$ where the last inequality is because $T-\StoppingMod \leq \TotalTime$ almost surely and $\underline{\CapRatio}$ is a constant by our assumption.
} We first note that \Cref{prop+stop+precise}, after some algebras, is equivalent to saying that 
\begin{equation}
    \P\Big[\TotalTime - \StoppingMod - \frac{1}{\underline{\CapRatio}} \geq x\Big] \leq \exp\left(
    -\frac{\underline{\CapRatio}^2x^2}{\TotalTime a^2}
    \right) + \sum_{\Locidx=1}^\Locnum \exp\left(-\frac{d_i^2}{2}(\TotalTime -x - \frac{1}{\underline{\CapRatio}})\right)
    \label{line:prob+tail}
\end{equation}
for any $ x\geq 0$. Assume, for the sake of simplicity, that $1/\underline{\CapRatio}$ is a positive integer (this makes us simplify the algebras). Similar to line \eqref{line:stop+algebra}, we have
\begin{equation*}
\begin{split}
\E\Big[(T-\StoppingMod - \frac{1}{\underline{\CapRatio}})^2\Big]
% RHS-1st 
&= \sum_{x=0}^{\TotalTime^2}\Pr\Big[(T-\StoppingMod - \frac{1}{\underline{\CapRatio}})^2 \geq x\Big]\\
%2nd
&= \sum_{x=0}^{\TotalTime^2}\Pr\Big[(T-\StoppingMod - \frac{1}{\underline{\CapRatio}}) \geq \sqrt{x}\Big]\\
% 3rd
&= \sum_{x=0}^{\TotalTime^2} \left\{
\exp\left(
-\frac{\underline{\CapRatio}^2 x}{\TotalTime a^2}
\right)
+ \sum_{\Locidx=1}^\Locnum \exp\left(- \frac{d_i^2}{2}(\TotalTime - \sqrt{x} - \frac{1}{\underline{\CapRatio}})\right)
\right\} \\
% 4th
&\leq 
    % term 1
\underbrace{
1 + \int_{0}^{\TotalTime^2}
\exp\left(
-\frac{\underline{\CapRatio}^2 x}{\TotalTime a^2}
\right) dx}_{(\clubsuit)} + 
    % term 2
\sum_{\Locidx=1}^\Locnum
\underbrace{
\int_{0}^{\TotalTime^2 +1} \exp\left(- \frac{d_i^2}{2}(\TotalTime - \sqrt{x} - \frac{1}{\underline{\CapRatio}})\right)dx}_{
\diamondsuit
}
\end{split}
\end{equation*}
The second line is justified because $T-\StoppingMod - \frac{1}{\underline{\CapRatio}}$ is non-negative almost surely.\footnote{Note that $\StoppingMod \geq \underline{\CapRatio}\TotalTime$ for every sample path. Hence, $\TotalTime-\StoppingMod$ must be greater than $\frac{1}{\underline{\CapRatio}}$ for all sufficiently large $\TotalTime$.} The third line follows from the tail bound \eqref{line:prob+tail}.
The last inequality follows since (i) $e(-a x)$ is a decreasing convex function for $x \in \R^+$ and $a>0$ and (ii) $e(\frac{d_i^2}{2}\sqrt{x})$ is an increasing concave function for all $x \geq 0$ and $d_i \leq 1$. It is straightforward to see that $\clubsuit \leq \BigO(\TotalTime)$. For $\diamondsuit$, we have
\begin{equation*}
\begin{split}
\diamondsuit &= 
% first line
\exp\left(- \frac{d_i^2}{2}(\TotalTime - \frac{1}{\underline{\CapRatio}})\right)\int_{0}^{\TotalTime^2 +1} \exp\left( \frac{d_i^2}{2} \sqrt{x}\right)dx \\
% 2nd
&= 
\exp\left(- \frac{d_i^2}{2}(\TotalTime - \frac{1}{\underline{\CapRatio}})\right)
\int_{0}^{\frac{d_i^4}{4}(\TotalTime^2+1)} \exp(\sqrt{u})\frac{4}{d_i^4}du\\
% 3nd
&=
\exp\left(- \frac{d_i^2}{2}(\TotalTime - \frac{1}{\underline{\CapRatio}})\right) \times \frac{4}{d_i^4}\left\{
2\exp\left(\sqrt{\frac{d_i^4}{4}(\TotalTime^2+1)}\right)\left(\sqrt{\frac{d_i^4}{4}(\TotalTime^2+1)}-1\right) + 2
\right\} \\
% fourth
&\leq 
\exp\left(- \frac{d_i^2}{2}(\TotalTime - \frac{1}{\underline{\CapRatio}})\right) \times \frac{8}{d_i^4}\left\{
\exp\left(\frac{d_i^2 T}{2} + \frac{d_i^2}{2}\right)\left(\frac{d_i^2 T}{2} + \frac{d_i^2}{2} - 1\right) + 2
\right\}\\
% fifth
&= \frac{8}{d_i^4}\left[
\exp\left(\frac{d_i^2}{2\underline{\CapRatio}} + \frac{d_i^2}{2}\right)\left(\frac{d_i^2\TotalTime}{2} + \frac{d_i^2}{2} - 1\right)+ 
2\exp\left(- \frac{d_i^2}{2}(\TotalTime - \frac{1}{\underline{\CapRatio}})\right) 
\right]\\
% last
&= \BigO(\TotalTime).
\end{split}
\end{equation*}

In the third line, we used $\int \exp(\sqrt{x})dx = 2 \exp(\sqrt{x})(\sqrt{x}-1)$. In the fourth line, we used $\sqrt{a+b} \leq \sqrt{a} + \sqrt{b}$ for any nonnegative scalars $a$ and $b$. The rest of the lines is a straightforward algebra. Hence, the proof is complete.
