# Supplementary material for: Dynamic Matching with Post-allocation Service and its Application to Refugee Resettlement
Source: arXiv:2410.22992 source file (2025-07-02)
Supplement: Supplementary file 3 [file apx+harvey+omitted.tex]

\subsubsection{Proof of \texorpdfstring{\Cref{lemma:last<=average+noise}}{}}\label{appendix:lemma:last<=average+noise} \hfill\\
For any arbitrary $k < s$, we have from Lemma \ref{lemma:average+convergence}
\begin{align}
    \sum_{t=s-k}^s [D(\boldsymbol{\nu}_t) -  D (\boldsymbol{\nu}_{s-k})] \leq \sum_{t = s-k}^s \frac{\eta_t G^2}{2\sigma} + \sum_{t= s-k}^s \hat{\mathbf{u}}_t \cdot (\boldsymbol{\nu}_t - \boldsymbol{\nu}_{s-k}) + 
    % additional terms
    \sum_{t=s-k+1}^{s} \left(\frac{1}{\eta_t} - \frac{1}{\eta_{t-1}}\right)V_h(\boldsymbol{\nu}_{s-k}, \boldsymbol{\nu}_t)
    . \label{equation:average(s-k)}
\end{align}
We first bound the last term as follows. Since the domain is bounded, the Bregman distance $V_h(\boldsymbol{\nu}_{s-k},\boldsymbol{\nu}_t)$ is bounded by some constant $D >0$. Let the step size be $\eta_t = c/\sqrt{t}$. Then we have
\begin{align}
\begin{split}
% first line 
\sum_{t=s-k+1}^{s} \left(\frac{1}{\eta_t} - \frac{1}{\eta_{t-1}}\right)V_h(\boldsymbol{\nu}_{s-k}, \boldsymbol{\nu}_t) &\leq D \sum_{t=s-k+1}^s \left(\frac{1}{\eta_t} - \frac{1}{\eta_{t-1}}\right) \\
&= Dc \sum_{t=s-k+1}^s \left(\sqrt{s} - \sqrt{k-1}\right)\\
% third 
&= Dc \frac{k-1}{\sqrt{s} + \sqrt{s-k+1}} \\ 
% fourth
&\leq Dc\frac{k+1}{\sqrt{s}}. \label{line:step+terms}
\end{split}
\end{align}

Let us define $S_k := \frac{1}{1+k}\sum_{t=s-k}^{s} D(\boldsymbol{\nu}_t)$. From line \eqref{equation:average(s-k)} and \eqref{line:step+terms}, 
\begin{align}
    S_k - D(\boldsymbol{\nu}_{s-k}) \leq \frac{1}{k+1}\sum_{t = s-k}^s \frac{\eta_t G^2}{2\sigma} + \frac{1}{k+1}\sum_{t= s-k}^s \hat{\mathbf{u}}_t \cdot (\boldsymbol{\nu}_t - \boldsymbol{\nu}_{s-k}) + O\left(\frac{1}{\sqrt{s}}\right).
    \label{ineq:(k+1)S_k}
\end{align}

Therefore, we can unwind $k S_{k-1}$ in a recursive form as follows:
\begin{align}
    kS_{k-1} &= \sum_{t=s-k+1}^s D(\boldsymbol{\nu}_t) \\
    % second line
    &= (k+1)S_k - D(\boldsymbol{\nu}_{s-k})\\
    % third line
    &= kS_k + S_k - D(\boldsymbol{\nu}_{s-k})\\
    % 5-th line 
    &= kS_k + \frac{1}{k+1}\sum_{t = s-k}^s \frac{\eta_t G^2}{2\sigma} + \frac{1}{k+1}\sum_{t= s-k}^s \hat{\mathbf{u}}_t \cdot (\boldsymbol{\nu}_t - \boldsymbol{\nu}_{s-k}) + O\left(\frac{1}{\sqrt{s}}\right) \quad \text{(Line \eqref{ineq:(k+1)S_k})}.
\end{align}
Dividing each side by $k$, we obtain
\begin{align}
    S_{k-1} \leq S_k + \frac{1}{k(k+1)}\sum_{t = s-k}^s \frac{\eta_t G^2}{2\sigma} + \frac{1}{k(k+1)}\sum_{t= s-k}^s \hat{\mathbf{u}}_t \cdot (\boldsymbol{\nu}_t - \boldsymbol{\nu}_{s-k}) + O\left(\frac{1}{k\sqrt{s}}\right).
\end{align}

By induction, we obtain
\begin{align}
    D(\boldsymbol{\nu}_s) = S_0 \leq S_{s/2} + 
    \underbrace{\sum_{k=1}^{s/2}\frac{1}{k(k+1)}\sum_{t = s-k}^s \frac{\eta_t G^2}{2\sigma}}_{:=\textsf{A}} +
    \underbrace{\sum_{k=1}^{s/2}\frac{1}{k(k+1)}\sum_{t= s-k}^s \hat{\mathbf{u}}_t \cdot (\boldsymbol{\nu}_t - \boldsymbol{\nu}_{s-k})}_{\textsf{B}} + 
    \underbrace{
    \sum_{k=1}^{s/2}O\left(\frac{1}{k\sqrt{s}}\right)}_{O\left(\frac{\log(s)}{\sqrt{s}}\right) \ (\text{Fact \ref{fact:1/i}})}
\end{align}
We first show that $\textsf{A} \leq O\left(\log(s)/\sqrt{s}\right)$ with $\eta_t = c/\sqrt{t}$. To see this,
\begin{align}
    % first line
    \textsf{A}  &= \sum_{k=1}^{s/2}\frac{1}{k(k+1)}\sum_{t = s-k}^s \frac{G^2 \eta_t}{2\sigma}\\
    % 2nd line
    &\leq \frac{G^2}{2\sigma}\sum_{k=1}^{s/2}\frac{1}{k(k+1)}(k+1)\eta_{s-k} \quad \text{($\eta_t$ is non-increasing in $t$)} \\
    % 3rd line
    &=\frac{G^2}{2\sigma}\sum_{k=1}^{s/2} \frac{1}{k} O\left( \frac{1}{\sqrt{s}}\right)\\
    % 4th line
    &= \frac{G^2}{2\sigma} O\left(\frac{\log(s)}{\sqrt{s}}\right) 
    \quad \text{(Fact \ref{fact:1/i})}.
\end{align} \par
We now turn our attention to term $B$. By chainging the order or summation, we have
\begin{align}
   \textsf{B} &=  \sum_{t=s/2}^s \sum_{k = s-t}^{s/2}  \frac{1}{k(k+1)}\hat{\mathbf{u}}_t \cdot (\boldsymbol{\nu}_t - \boldsymbol{\nu}_{s-k}) \\
   &= \sum_{t=s/2}^s \sum_{j = s/2}^t \frac{1}{(s-j)(s-j+1)} 
   \hat{\mathbf{u}}_t \cdot (\boldsymbol{\nu}_t - \boldsymbol{\nu}_{j}) \\
   &= \sum_{t=s/2}^s \hat{\mathbf{u}}_t \cdot 
   \underbrace{
   \left[
   \sum_{j = s/2}^t \frac{1}{(s-j)(s-j+1)}  (\boldsymbol{\nu}_t - \boldsymbol{\nu}_{j})
   \right]}_{:=\boldsymbol{\omega}_t}
\end{align}
where the second line follows from change of variable $j = s-k$.
This completes the proof.

\subsubsection{Proof of \texorpdfstring{\Cref{lemma:first+term}}{}}\label{appendix:lemma:first+term}\hfill\\
From Lemma \ref{lemma:average+convergence}, we have
\begin{align}
% LHS
\sum_{t=s/2}^s[D(\boldsymbol{\nu}_t) - D(\boldsymbol{\nu}^*)] 
\leq 
% RHS 
\sum_{t={s/2}}^s \frac{\eta_t G^2}{2\sigma} + 
% additional terms 
\sum_{t=s/2 +1}^{s} \left(\frac{1}{\eta_t} - \frac{1}{\eta_{t-1}}\right)V_h(\boldsymbol{\nu}, \boldsymbol{\nu}_t) +
\frac{1}{\eta_{s/2}}V_h(\boldsymbol{\nu^*}, \boldsymbol{\nu}_{s/2}) + 
\sum_{t={s/2}}^s \hat{\mathbf{u}}_t\cdot(\boldsymbol{\nu}_t - \boldsymbol{\nu}^*) 
\end{align}
Since we assume that $G$ and $\sigma$ is constant, we will omit the dependence on these two primitives. From Fact \ref{fact:1/sqrt(i)}, we have
\begin{align}
    \sum_{t=s/2}^s \eta_t = \sum_{t=s/2}^s O(1/\sqrt{t}) = O(\sqrt{s}).
\end{align}
In the similar way, by using the bounded domain and the telescoping sum of $\frac{1}{\eta}_t - \frac{1}{\eta_{t-1}}$,
one can bound the second term by $O(\sqrt{s})$ 
The third term is again $O(\sqrt{s})$ due to the bounded domain assumption. Finally, note that the $\E[\mathbf{\hat{u}}_t| \History_{t-1}] = 0 $ and hence the last term is the martingale with respect to $\History_t$. Due to the bounded domain assumption, we have $\lVert \boldsymbol{\nu}_t - \boldsymbol{\nu}^*\rVert \leq O(1)$ and therefore $\sum_{t=s/2}^s \lVert \boldsymbol{\nu}_t - \boldsymbol{\nu}^*\rVert^2 \leq O(s)$. Invoking Fact \ref{fact:azuma}, we can bound the last term as $O(\sqrt{s\log(1/\delta)})$ with probabiltiy $1-\delta$.

%%%%%%%%%%%%%%%%%%%%%%%%%%%%%%%%%%
\subsubsection{Proof of \texorpdfstring{Claim \ref{claim:omega}}{}}\label{appendix:claim:omega}\hfill\\
   Define $\alpha_j := \frac{1}{(s-j)(s-j+1)}$ and $A := \sum_{j=s/2}^{t} \alpha_j$. We also recall that
    \begin{align}
        \boldsymbol{\omega}_t = \sum_{j=s/2}^t \alpha_j (\boldsymbol{\nu}_t - \boldsymbol{\nu}_j ) = \sum_{j=s/2}^{t-1} \alpha_j (\boldsymbol{\nu}_t - \boldsymbol{\nu}_j )
    \end{align}
Hence, we have
\begin{align}
    % first line 
    \lVert \boldsymbol{\omega}_t \rVert_2^2 &= A^2 \bigg\lVert 
    \sum_{j=s/2}^{t-1}\frac{\alpha_j}{A}(\boldsymbol{\nu}_t - \boldsymbol{\nu}_j)
    \bigg\rVert_2^2\\
    % 2nd line 
    &\leq A^2  \sum_{j = s/2}^{t-1} \frac{\alpha_j}{A} \lVert 
    \boldsymbol{\nu}_t - \boldsymbol{\nu}_j\rVert_2^2 \quad \text{(Convexity of $\lVert \cdot \rVert_2^2$)} \\ 
    % 3rd line
    &= A \sum_{j = s/2}^{t-1} \alpha_j \lVert 
    \boldsymbol{\nu}_t - \boldsymbol{\nu}_j\rVert_2^2 \\
    % last line 
    &\leq \frac{1}{s-t+1}\sum_{j = s/2}^{t-1} \alpha_j \lVert 
    \boldsymbol{\nu}_t - \boldsymbol{\nu}_j\rVert_2^2 \quad \text{(Fact \ref{fact:partial+fraction })}.
\end{align}

\subsubsection{Proof of \texorpdfstring{ \Cref{lemma:bound+distance}}{}}\label{appendix:lemma:bound+distance}\hfill\\

From Claim \ref{claim:omega} and Lemma \ref{lemma:bound+distance}, we have $\sum_{t=s/2}^s \lVert 
\omega_t\rVert_2^2 \leq \Lambda_1 + \Lambda_2 + \Lambda_3$ where
\begin{align}
    % Lambda1
    \Lambda_1 &:= \frac{2G}{\sigma^2}\sum_{t=s/2}^s \frac{1}{s-t+1}\sum_{j=s/2}^{t-1}\alpha_j \sum_{i=j}^{t-1} \eta_i^2 \\
    % Lambda2
    \Lambda_2 &:= \frac{2}{\sigma} \sum_{t=s/2}^{s}\frac{1}{s-t+1}\sum_{j=s/2}^{t-1} \alpha_j \sum_{i=j}^{t-1} \eta_i (D(\boldsymbol{\nu}_j) - D(\boldsymbol{\nu}_i))\\
    % Lambda3
    \Lambda_3 &:= \frac{2}{\sigma} \sum_{t=s/2}^{s}\frac{1}{s-t+1}\sum_{j=s/2}^{t-1}\alpha_j \sum_{i=j}^{t-1} \eta_i \mathbf{\hat{u}}_i(\boldsymbol{\nu}_i - \boldsymbol{\nu}_j).
\end{align} We bound each term in the following.

\begin{claim}\label{claim:Lambda1}
    $\Lambda_1 \leq O\left(\dfrac{\log^2(s)}{s}\right)$.
\end{claim}
{\bf Proof of Claim \ref{claim:Lambda1}.}
\begin{align}
% first line
\Lambda_1 &:= \frac{2G}{\sigma^2}\sum_{t=s/2}^s \frac{1}{s-t+1}\sum_{j=s/2}^{t-1}\alpha_j \sum_{i=j}^{t-1} \eta_i^2\\
% 2nd line
&\leq  \frac{2G}{\sigma^2} \sum_{t=s/2}^s \frac{1}{s-t+1}\sum_{j=s/2}^{t-1}\alpha_j (s-j)\eta_{s/2}^2  \quad \text{($\eta_i$ non-increasing in $i \geq s/2$) }\\
% 3rd line
&= \frac{2G \eta_{s/2}^2}{\sigma^2}\sum_{t=s/2}^s \frac{1}{s-t+1}\sum_{j=s/2}^{t-1} \frac{1}{s-j+1} \\
% 4th line
&\leq \frac{2G \eta_{s/2}^2}{\sigma^2}\O(\log^2 (s)) \quad \text{(Fact \ref{fact:1/i})}\\
% last line
&\leq O\left(\frac{\log^2(s)}{s}\right) \quad \text{($\eta_{s/2} = O(1/\sqrt{s})$)}
\end{align}
\hfill\halmos

\begin{claim}\label{claim:Lambda2}
    $\Lambda_2 \leq O\left(\dfrac{\log^2(s)\sqrt{\log(1/\delta)}}{s}\right)$ with probability at least $1-\delta$.
\end{claim}
{\bf Proof of Claim \ref{claim:Lambda2}}
We first write $\Lambda_2$ as 
\begin{align}
\Lambda_2 = \frac{2}{\sigma}\sum_{t=s/2}^{s} \frac{1}{s-t+1}\sum_{j=s/2}^{t-1}\alpha_j \sum_{i=j}^{t-1} \eta_i (F_j - F_i) \quad \text{where $F_i := D(\boldsymbol{\nu}_i) - D(\boldsymbol{\nu}^*)$}. \label{eq:Lambda2+F}
\end{align}
Our plan will be the following: we will first write $\Lambda_2$ \eqref{eq:Lambda2+F} as
\begin{align}
    \Lambda_2 = \frac{2}{\sigma}\sum_{a=s/2}^{s-1} r_a F_a \label{eq:Lambda2+r}
\end{align} 
for some $r_a \leq O\left(\frac{\log(s)}{s^{1.5}}\right)$. This will enable us to bound $\Lambda_2$ as 
\begin{align}
    \Lambda_2 \leq O\left(\frac{\log(s)}{s^{1.5}}\right) \sum_{a=s/2}^{s-1} F_a. \label{eq:Lambda2+average}
\end{align}
Finally, note that $\sum_{a=s/2}^{s-1}$ is exactly related to the average convergence result in Lemma \ref{lemma:average+convergence}. Similar to the proof of Lemma \ref{lemma:first+term}, we will bound this term by $O\left(\log(1/\delta)/\sqrt{s}\right)$ with probability at least $1-\delta$ using Azuma's inequality. \par 
Now let us investigate the coefficient $r_a$ in line \eqref{eq:Lambda2+r}. 
\begin{align}
    r_a = \underbrace{\sum_{t=a+1}^{s}\frac{1}{s-t+1}\sum_{i=a}^{t-1}\alpha_a \eta_i}_{\textsf{Pos}} - 
    \underbrace{
    \sum_{t= a+1}^{s} \frac{1}{s-t+1}\sum_{j=s/2}^{a} \alpha_j \eta_a}_{\textsf{Neg}}
    \label{eq:r+a}
\end{align}
To see this, the indices contributing to the positive coefficient for $F_a$ must satisfy $j=a$ and $a \leq i \leq t-1$ in line \eqref{eq:Lambda2+F}. In the similar way, the indices providing a negative coefficient for $F_a$ must satisfy $i=a$ and $j \leq a \leq t-1$. Collecting all of the positive and negative coefficients for $F_a$ gives line \eqref{eq:r+a}. \par
We now observe that $r_a \leq  O\left(\frac{\log(s)}{s^{1.5}}\right)$ for all $ s/2 \leq a \leq s-1$ in the following. 
% positive part 
\begin{align*}
% first line
\textsf{Pos}&\leq \sum_{t=a+1}^s \frac{1}{s-t+1}\alpha_a \frac{2c(t-a)}{\sqrt{t-1} + \sqrt{a-1}} \quad \text{(Fact \ref{fact:1/sqrt(i)})} \\
% 2nd line
&\leq \sum_{t=a+1}^s \frac{1}{s-t+1}\alpha_a \frac{2c(t-a)}{\sqrt{a-1} + \sqrt{a-1}} \quad \text{($t \geq a-1$)}\\
% 3rd line
&= \sum_{t=a+1}^s \frac{1}{s-t+1}\frac{1}{(s-a)(s-a+1)}\frac{c(t-a)}{\sqrt{a-1}} \quad \text{($t \geq a-1$)}\\
% 4th line
&\leq \sum_{t=a+1}^s \frac{1}{s-t+1}\frac{c}{(s-a)\sqrt{a-1}} \quad \text{($t -a \leq s-a+1$)}\\
% 5th line
&\leq \frac{c\sqrt{a}}{s-a}\sum_{t=a+1}^s \frac{1}{(s-t+1)(a-1)}
\end{align*}

% negative part 
\begin{align*}
\textsf{Neg} &= \sum_{t=a+1}^s \frac{1}{s-t+1}\frac{c}{\sqrt{a}}\left(\frac{1}{s-a} - \frac{1}{s/2+1}\right) \quad \text{(Fact \ref{fact:partial+fraction })}\\
% 2nd line
&= \sum_{t=a+1}^s \frac{1}{s-t+1}\frac{c}{\sqrt{a}}\frac{a+1-s/2}{(s-a)(s/2+1)}\\
% 3rd line
&= \frac{2c\sqrt{a}}{(s+2)(s-a)}\sum_{t=a+1}^{s}\frac{1}{s-t+1}\left(1 - \frac{s-2}{2a}\right)
\end{align*}
Combining, we have
\begin{align*}
% first line
    r_a &= \textsf{Pos} - \textsf{Neg}\\
% 2nd line
    &\leq \frac{c\sqrt{a}}{(s-a)}\sum_{t=a+1}^s\left(\frac{1}{s-t+1}\right)\left[
    \frac{1}{a-1} - \frac{2}{s+2}\left(
    1 - \frac{s-2}{2a}
    \right)
    \right]\\
% third line
    &= \frac{c\sqrt{a}}{(s-a)}\sum_{t=a+1}^s\left(\frac{1}{s-t+1}\right)\left[
    \frac{s+2 - 2(a-1) + \frac{2(a-1)(s-2)}{2a}}{(a-1)(s+2)}
    \right]\\
% 4th line 
    &\leq \frac{c\sqrt{a}}{(s-a)}\sum_{t=a+1}^s\left(\frac{1}{s-t+1}\right)\left[
    \frac{2(s-a) + 2}{(a-1)(s+2)}
    \right]\\
% 5th
&\leq \frac{c\sqrt{a}}{(s-a)}\sum_{t=a+1}^s\left(\frac{1}{s-t+1}\right)\left[
    \frac{4(s-a)}{(a-1)(s+2)}
    \right] \quad \text{($s-a \geq 1$)}\\
% 6th
&= \frac{4c\sqrt{a}}{(a-1)(s+2)}\sum_{t=a+1}^s\left(\frac{1}{s-t+1}\right)\\
&\leq O\left(\frac{\log(s)}{s^{1.5}}\right) \text{($a \geq s/2$ and Fact \ref{fact:1/i})}.
\end{align*}
 \par 
Since $\sigma$ is constant and $r_a \leq O\left(\frac{\log(s)}{s^{1.5}}\right)$ for all $s/2 \leq  s-1$, we can now bound $\Lambda_2$ as line \eqref{eq:Lambda2+average}. We can further expand line \eqref{eq:Lambda2+average} as follows:

\begin{align}
\Lambda_2 \leq O\left(\frac{\log(s)}{s^{1.5}}\right)\left[
% term 1 
\underbrace{
\sum_{t=s/2}^{s-1}\frac{\eta_t G^2}{2\sigma}}_{\leq O(\sqrt{s})} + 
% term 2
\underbrace{
\frac{1}{\eta_{s/2}} V_h(\boldsymbol{\nu}^*, \boldsymbol{\nu}_{s/2})
}_{\leq O(\sqrt{s})}
% term 3
\underbrace{
 + \sum_{t=s/2}^{s-1} \mathbf{\hat{u}}_t \cdot (\boldsymbol{\nu}_t - \boldsymbol{\nu}^*)}_{\leq \sqrt{s\log(1/\delta)} \text{\ w.p $1-\delta$}}
 % term 4 
 \underbrace{
 + \sum_{t=s/2+1}^{s-1}
 \left(
 \frac{1}{\eta_t} - \frac{1}{\eta_{t-1}} \right)V_h(\boldsymbol{\nu}^*, \boldsymbol{\nu}_t)}_{O(\sqrt{s})}
\right]
\end{align}
The bound for the first follows from $\eta_i = O(c/\sqrt{i})$ and Fact \ref{fact:1/sqrt(i)}. The second term follows again $\eta_i = O(c/\sqrt{i})$ and bounded domain assumption. Finally, note that the $\E[\mathbf{\hat{u}}_t| \History_{t-1}] = 0 $ and hence the third term is the martingale with respect to $\History_t$. Due to the bounded domain assumption, we have $\lVert \boldsymbol{\nu}_t - \boldsymbol{\nu}^*\rVert \leq O(1)$ and therefore $\sum_{t=s/2}^s \lVert \boldsymbol{\nu}_t - \boldsymbol{\nu}^*\rVert^2 \leq O(s)$. Invoking Fact \ref{fact:azuma} (Azuma's inequality), we can bound the third term as $O(\sqrt{\log(1/\delta)/s})$ with probability $1-\delta$. The Last term is again $O(\sqrt{t}$ since the domain is bounded (and therefore so is the Bregman distances) as well as $\eta_t = \frac{c}{\sqrt{t}}$. This completes the proof.
\hfill\halmos

\begin{claim}\label{claim:Lambda3}
    $\Lambda_3 \leq \frac{2}{\sigma}\sum_{i=s/2}^{s-1} \tilde{\alpha}_i (\mathbf{\hat{u}}_i \cdot
\boldsymbol{\omega}_i)$ where $\tilde{\alpha}_i = \eta_i\sum_{j=i+1}^{s} \frac{1}{s-i+1}$
\end{claim}
{\bf Proof of \ref{claim:Lambda3}}
\begin{align}
% first line
\Lambda_3 &=  \frac{2}{\sigma} \sum_{t=s/2}^{s}\frac{1}{s-t+1}\sum_{j=s/2}^{t-1}\alpha_j \sum_{i=j}^{t-1} \eta_i \mathbf{\hat{u}}_i\cdot(\boldsymbol{\nu}_i - \boldsymbol{\nu}_j) \\
% second line
&= \frac{2}{\sigma} \sum_{t=s/2}^{s}\frac{1}{s-t+1}\sum_{i=s/2}^{t-1}\sum_{j=s/2}^{i
} \eta_i \alpha_j \mathbf{\hat{u}}_i\cdot(\boldsymbol{\nu}_i - \boldsymbol{\nu}_j) \quad{\text{(change the order of summation)}}\\
% 3rd line
&= \frac{2}{\sigma}\sum_{t=s/2}^{s}\frac{1}{s-t+1}\sum_{i=s/2}^{t-1}\eta_i \mathbf{\hat{u}}_i\cdot \left(
\underbrace{
\sum_{j=s/2}^{i} \alpha_j(\boldsymbol{\nu}_i - \boldsymbol{\nu}_j)}_{=\boldsymbol{\omega}_{i}}
\right) \\
&= \frac{2}{\sigma}\sum_{t=s/2}^{s}\frac{1}{s-t+1}\sum_{i=s/2}^{t-1}\eta_i \mathbf{\hat{u}}_i\cdot \boldsymbol{\omega}_i \\ 
&= \frac{2}{\sigma}\sum_{i=s/2}^{s-1} 
\underbrace{
\left(
\eta_i\sum_{t=i+1}^{s}\frac{1}{s-t+1}
\right)}_{

:= \tilde{\alpha}_i}
(\mathbf{\hat{u}}_i \cdot
\boldsymbol{\omega}_i) \quad{\text{(change the order of summation)}} \\
&= \frac{2}{\sigma}\sum_{i=s/2}^{s-1} \tilde{\alpha}_i (\mathbf{\hat{u}}_i \cdot
\boldsymbol{\omega}_i)
\end{align}
\hfill\halmos

Combining Claim \ref{claim:Lambda1}-\ref{claim:Lambda3}, we obtain
\begin{align}
    \sum_{t=s/2}^{s} \lVert \boldsymbol{\omega}_t \rVert_2^2 \leq \frac{2}{\sigma}\sum_{t=s/2}^{s-1} \tilde{\alpha}_t (\mathbf{\hat{u}}_t \cdot \boldsymbol{\omega}_t) + O\left(\frac{\log^2(s)\sqrt{\log(1/\delta)}}{s}\right)
\end{align}
where $\tilde{\alpha}_t = \eta_t \sum_{j=t+1}^{s}\frac{1}{s-t+1}$. By defining $d_t = \frac{1}{2}(\mathbf{\hat{u}}_t \cdot \boldsymbol{\omega}_t)$, we obtain 
\begin{align}
\sum_{t=s/2}^{s} \lVert \boldsymbol{\omega}_t \rVert_2^2 \leq \sum_{t=s/2}^{s-1}\tilde{\alpha}_t (\mathbf{\hat{u}}_t \cdot \boldsymbol{\omega}_t) + R\sqrt{\log(1/\delta)}
\end{align}
where $R = O\left(\frac{\log^2(s)}{s}\right)$ and $\tilde{\alpha}_t := \frac{4}{\sigma}\eta_t \sum_{j=t+1}^{s}\frac{1}{s-t+1} > 0$. The proof is complete by noting that $\max_{s/2 \leq t \leq s}\tilde{\alpha}_t \leq O\left(\frac{\log(s)}{\sqrt{s}}\right) = O(\sqrt{R})$. 

\hfill\halmos
