# Supplementary material for: Dynamic Matching with Post-allocation Service and its Application to Refugee Resettlement
Source: arXiv:2410.22992 source file (2025-07-02)
Supplement: Supplementary file 4 [file apx+near+part+b+reward.tex]

\begin{comment}
\subsection{Proof of 
\texorpdfstring{\Cref{lemma:all+time+reward}}{}}\label{apx+all+time+reward}    
\end{comment}
\subsection{Proof of 
\texorpdfstring{\Cref{lemma:Z+lower}}{}}\label{apx+all+time+reward} 
%\hfill\\
The proof follows similar steps for proving \Cref{lemma:goal} in Appendix \ref{apx+B-2}. For brevity, we only highlight a main difference from the proof. As we consider a one-dimensional example with capacity ratio $\CapRatio =0.5$, we omit the subscript for $\Locidx$. Fix a sample path of rewards $w_1,...w_T$. Let $\Decision_\Timeidx$ be the decision for arrival $\Timeidx$. Because the algorithm is unconstrained by the hard capacity constraint until $\Timeidx \leq \CapRatio \TotalTime$, the optimality criterion of the algorithm implies that
\begin{equation*}
\sum_{\Tauidx=1}^\Timeidx (\Weight_\Tauidx - \DualOver_\Tauidx - \Indicator[\Target_\Tauidx=0]\DualHard_\Tauidx)\cdot\Decision_\Tauidx + \CapRatio\cdot(\DualOver_\Tauidx + \DualHard_\Tauidx) \geq \sum_{\Tauidx=1}^\Timeidx (\Weight_\Tauidx - \DualOver_\Tauidx - \Indicator[\Target_\Tauidx=0]\DualHard_\Tauidx)\Decision_\Tauidx ^* + \CapRatio\cdot(\DualOver_\Tauidx + \DualHard_\Tauidx). 
\end{equation*}
for any fixed $\Timeidx \leq \CapRatio \TotalTime$ and any alternative decision $\Decision^*_\Tauidx \in \FeasibleSet{\Target_\Tauidx}$. Now take the same alternative decision as defined in line \eqref{line:z+tau+star}. By following the identical steps up to line \eqref{line:upto}, we can show that, with probability at least $1-\delta$,
\begin{equation*}
\OverCost\left(\sum_{\Tauidx=1}^\Timeidx \Decision_{\Tauidx} - \Timeidx\CapRatio\right)_{+}
% RHS-1st 
\leq 
%\SLedit{
\nu^*\left(
 \sum_{\Tauidx=1}^\Timeidx \Decision_{\Tauidx} - \Timeidx\CapRatio
\right)
%} 
+ M\sqrt{t\log(1/\delta)} 
\end{equation*}
where $\nu^*$ is the (optimal) dual variable corresponding to the capacity constraint in the optimization problem \eqref{line:const}.\footnote{The optimization problem admits a feasible solution for every sample path because there is no tied case.} For this instance, as we discuss in \Cref{example:stable}, the dual variable $\nu^*$ for each sample path $\Weight_1,...,\Weight_\Timeidx$ is the sample median of the rewards. Because the support of the reward is bounded away from zero, there exists a constant $\underline{\nu}>0$ such that $\nu^* \geq \underline{\nu}$.\footnote{One can make this argument more precise by incorporating the concentration of $\nu^*$. By the property of the uniform random variable on interval $(0,1)$, the sample median of $(w_1,...w_\Timeidx)$ follows Beta($t/2+1$, $t/2+1$) distribution (see, for example, Example 5.4.5 of \cite{casella2021statistical}). Hence, the mean of $\nu^*$ is $1/2$ and the variance is $\Theta(1/\Timeidx)$. Hence, for large enough $\Timeidx$, the variance of $\nu^*$ is small enough to ensure that $\nu^*$ is bounded above some fixed constant $\underline{\nu}$ with high probability. The result incorporating this detail only changes the result of \Cref{thm:last+iterate} in a minor manner. For the sake of brevity, we omit such details in the proof. } 
Hence, dividing the above inequality by $\nu^*$ and defining the constant $\kappa := \frac{M}{\underline{\nu}}$,
we conclude that
\begin{equation*}
 \sum_{\Tauidx=1}^\Timeidx \Decision_{\Tauidx} \geq  \Timeidx\CapRatio - \kappa\sqrt{t\log(1/\delta)}
\end{equation*}
with probability at least $1-\delta$.
