# Supplementary material for: Dynamic Matching with Post-allocation Service and its Application to Refugee Resettlement
Source: arXiv:2410.22992 source file (2025-07-02)
Supplement: Supplementary file 5 [file apx+nonunit+case+study.tex]

{
\color{blue}
\section{Numerical Results with Varying Case Size}\label{apx+non+unit+numerics}

Our main case study (Section~\ref{sec:numerics}) assumed unit-size capacity consumption per case. This setup is largely aligned with resettlement programs in some countries, such as Switzerland, where capacities are defined at the case level. In contrast, U.S. resettlement programs set affiliate capacity based on individuals. Consequently, each case consumes a different number of capacity units depending on its family size. In this section, we provide additional numerical results that incorporate varying family sizes and individual-level capacity consumption.  

Our model and algorithms naturally extend to accommodate such variation. In particular, this setting corresponds to a special case of the generalized model introduced in \Cref{apx+non+unit+size}, which allows each case to consume multiple units of one or more types of static resources. We build on the generalized model in Section~\ref{apx+non+unit+size} for the numerical study with varying family size. Specifically, we augment each case~$t$ with a family size~$n_t$.\SLcomment{\@Elisabeth; please let me know if we were approved to report summary statistics regarding $n_t$ (e.g., average).} The employment probability vector~$\mathbf{w}_t$ and target affiliate~$\Target_t$ remain unchanged from our base case study in \Cref{sec:numerics}. Capacity~$c_i$ is set to the actual number of individuals placed at affiliate~$i$ by our partner agency. Each case~$t$ consumes~$n_t$ units of this capacity. We modify backlog dynamics accordingly as described in Equation~\eqref{eq:backlog+generalized} in \Cref{subsec:generalized+model}. We retain the deterministic service model with per-period service rate $\rho_i = c_i / T$.  \texttt{RO-Learning} is instantiated as \CAM{}, a modification of \CA{} from Section~\ref{subsec+generalized+algos}, with an additional constraint that each case must be matched to an actual affiliate. Similarly, \CO{} is modified analogously to \COM{}, as described in Section~\ref{subsec+generalized+algos}. 

Table~\ref{table:varying-size-simulation} reports results under penalty parameters $\alpha = 3$ and $\gamma = 5$ (the same values used  in Figure~\Cref{fig:performance}). We observe that \texttt{RO-Learning}, our main proposed algorithm, continues to show a substantial improvement in employment outcomes and average backlog compared to the current practice (\texttt{Actual}). Relative to \texttt{Sampling}, \texttt{RO-Learning} achieves a comparable employment rate (a relative loss of less than 5\%) while incurring substantially lower over-allocation (22--47\% reduction) and average backlog (more than 20\% reduction). Finally, although \COM{} generally underperforms both \texttt{Sampling} and \texttt{RO-Learning}—which both utilize backlog information—it still yields a notable improvement compared to the current practice (\texttt{Actual}) in employment outcomes and average backlog,  despite not using any backlog information. Overall, this numerical result shows that our proposed algorithms can serve as effective alternatives to the benchmarks even when we incorporate the varying case size. 

\begin{table}[htp]
    \centering
    \caption{
    Numerical performance for year 2015 (2016, resp.) with varying family size under penalty parameters $\boldsymbol{\alpha = 3}$ and $\boldsymbol{\gamma = 5}$. %Backlog and over-allocation reflect individual-level capacities.
    }
    \label{table:varying-size-simulation}
    \begin{tabular}{@{}lccc@{}}
        \toprule
        & \makecell{\textbf{Employment}  \textbf{Rate (\%)}} 
        & \makecell{\textbf{Total} \textbf{Over-} \textbf{allocation}} 
        & \makecell{\textbf{Average}  \textbf{Backlog}} \\
        \midrule
        \texttt{Actual}        & 37.3 (37.9) & 0 (0)             & 641.2 (996.8) \\
        \texttt{Sampling}      & 45.7 (47.5) & 308.4 (366.2)     & 526.9 (792.6) \\
        \texttt{RO-Learning}   & 44.3 (45.2) & 239 (194)         & 414.3 (615.5) \\
        \COM{} & 45.5 (45.2) & 284 (314) & 542.9 (852.7) \\
        \bottomrule
    \end{tabular}
\end{table}

}
