# Supplementary material for: Dynamic Matching with Post-allocation Service and its Application to Refugee Resettlement
Source: arXiv:2410.22992 source file (2025-07-02)
Supplement: Supplementary file 6 [file apx+numerics+additional+benchmarks.tex]

\subsection{Additional Numerical Results with Proxies for the Current Pratices}\label{apx+case+additional+benchmarks}

In this section we compare the performance of \texttt{Learning} and \texttt{Sampling} to two additional benchmarks. First, we consider the \texttt{Random} benchmark in which a free case arriving at time $t$ is allocated, at random, to one of the affiliates with remaining capacity, in proportion to the affiliates' remaining capacity. For example, if there are two affiliates left with remaining capacity, one with capacity 4 and one with capacity 6, the current case is matched to the first affiliate with probability 40\%. 

Second, we consider the \texttt{Min \Backlog{}} benchmark, in which a free case arriving at time $t$ is allocated to the affiliate with the smallest buildup at time $t$. In the case of ties, an affiliate is chosen at random (in proportion to remaining capacity) among those with minimum buildup. 

Figure \ref{fig:additional-benchmarks} shows the results. For the \texttt{Random} and \texttt{Min Buildup} benchmarks, results are shown across 100 random instances.

\begin{figure}[t]
  \begin{subfigure}{\linewidth}
    \centering
    \includegraphics[width=\linewidth]{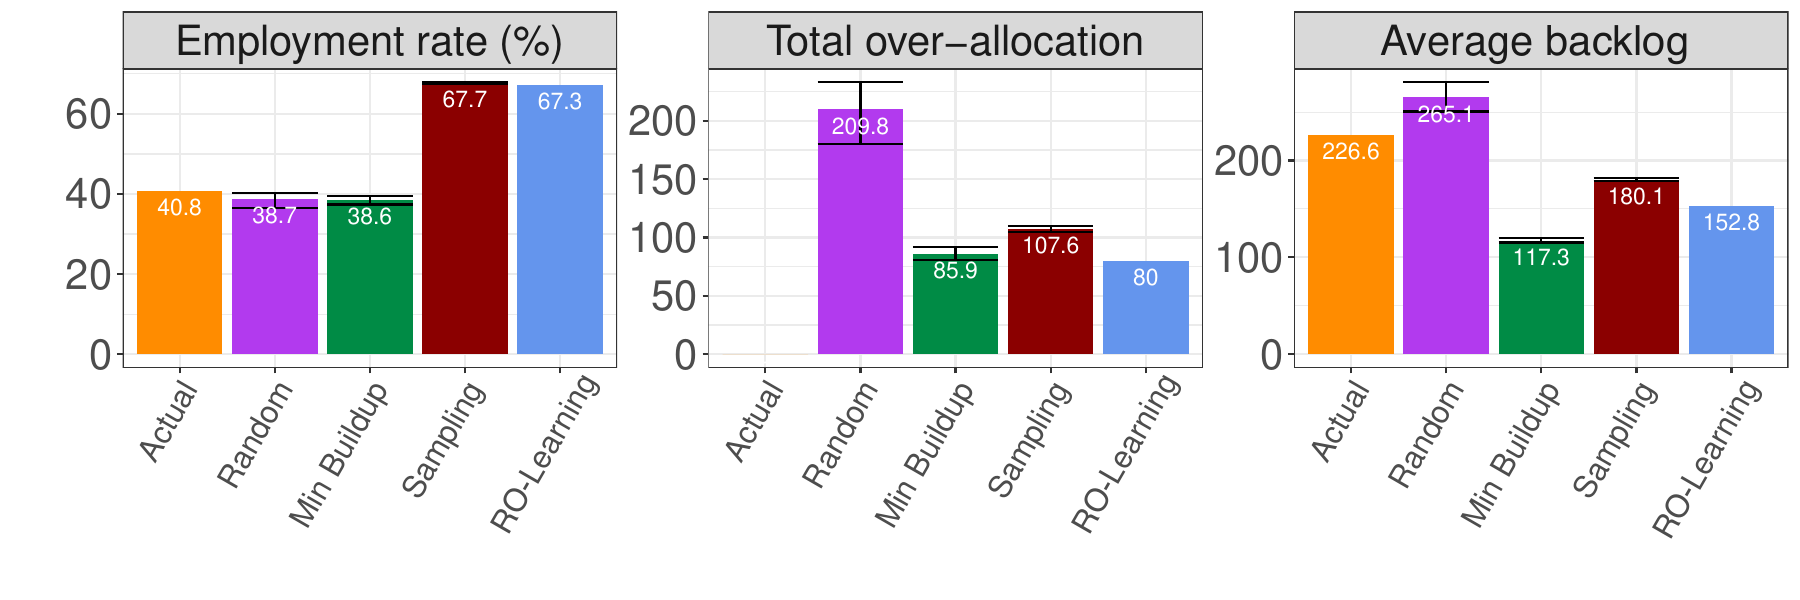}
    \caption{Year 2015}
    %\label{fig:performance:subfig1}
  \end{subfigure}

    \begin{subfigure}{\linewidth}
    \centering
    \includegraphics[width=\linewidth]{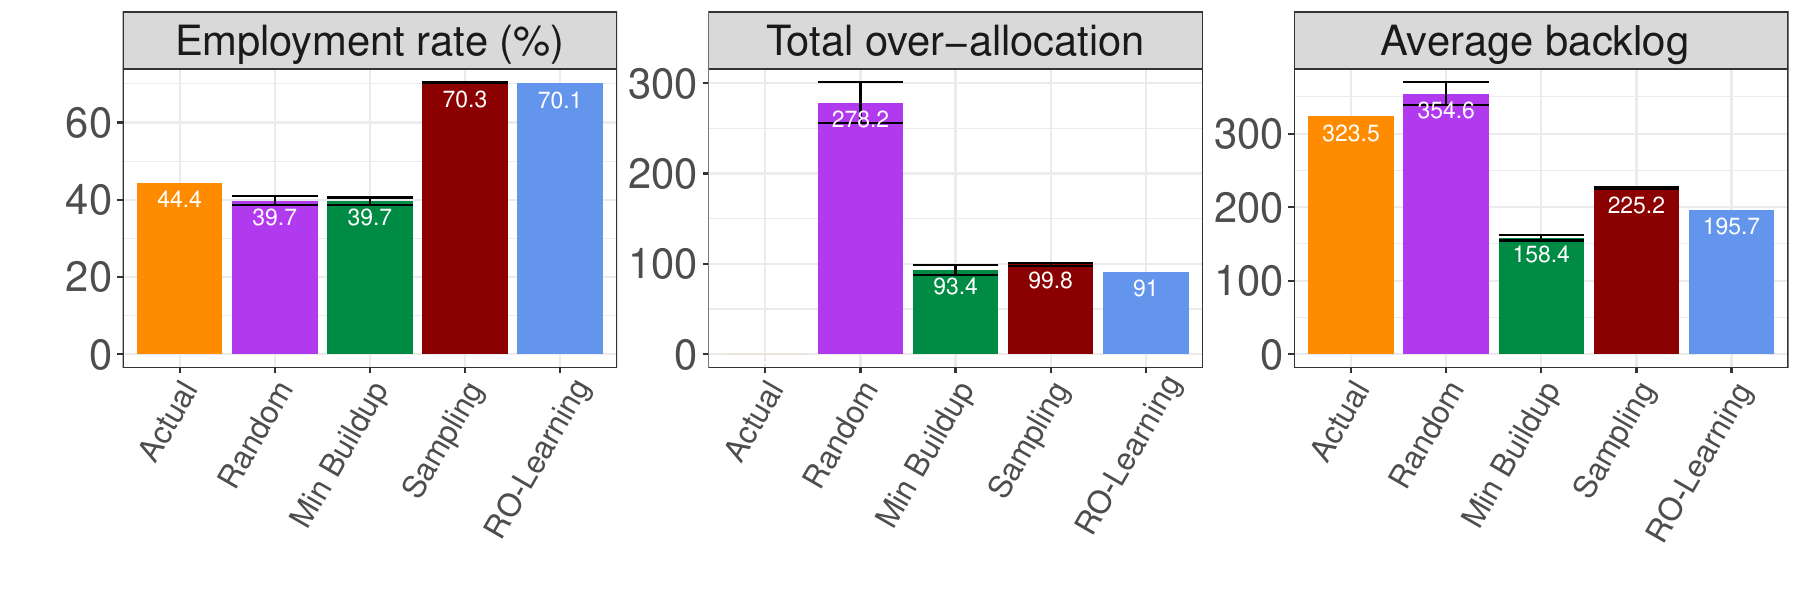}
    \caption{Year 2016}
    %\label{fig:performance:subfig2}
  \end{subfigure}
    \caption{Performance of the algorithms on real data of a major resettlement agency in the US. Here we present the result for cost parameters $\OverCost=3$ and $\BuildUpCost=5$. The employment rate is the total employment outcome normalized by the total number of free cases. The average \backlog{} is $\frac{1}{{\TotalTime}}\sum_{\Timeidx=1}^\TotalTime\sum_{\Locidx=1}^m \BuildUp_{\Timeidx, \Locidx}$. For the algorithms with randomness, the error bars show the maximum and minimum values achieved over 100 random simulations for Random and Min Buildup, and 5 simulations for Sampling.}
    \label{fig:additional-benchmarks}
    %\SLcomment{Could you please check the build-up for the sampling and Learning? I remember, for year 2015, it was 2.7-8 or something like it for our algo and the value for sampling was 15\% higher. Plus, rather than normalizing by $m$, I think it might be better to show $\frac{1}{\TotalTime}\sum_{\Timeidx=1}^\TotalTime \BuildUp_{\Timeidx, \Locidx}$. Let me know your thoughts! }\EPcomment{the numbers for Actual, Sampling, and Learning have slightly changed because there was an error with $M$ which I fixed. I was using $M=52$ which is the number of unique locations across 2014-2016, instead of using each years' $M$ separately (which is 45 for 2015 and 49 for 2016). I'll change the figures now that we don't divide by $M$ and this will no longer be a relevant issue! I also fixed the caption so that the equation is correct.}\SLcomment{Thanks!! This comment is cleared.}
\end{figure}
