# Supplementary material for: Dynamic Matching with Post-allocation Service and its Application to Refugee Resettlement
Source: arXiv:2410.22992 source file (2025-07-02)
Supplement: Supplementary file 7 [file apx+numerics+additional+results.tex]

\subsection{Additional Numerical Results for \texttt{RO-Learning} versus \texttt{Sampling}}\label{apx+case+additional+results}
%\SLcomment{changed the section titles}
In this subsection, we present A more extensive case study for a broader range of the cost parameters $\OverCost$ and $\BuildUpCost$. In Figure \ref{fig:more+case}, we display the results of the placement outcome for $\OverCost \in \{1,2,..,5\}$ and $\BuildUpCost \in \{0,1,...,10\}$. In each panel, we display the trajectory of the outcome metrics of fixed $\OverCost$ (label of the penal) and varying $\BuildUpCost$. Here, the point \texttt{Opt-Emp} is the outcome achieved by the surrogate primal problem (see \Cref{def:primal+surrogate}), which does not incur any over-allocation when $\OverCost\geq 1$. \par 

We first note that \texttt{RO-Learning} consistently improves upon \texttt{Actual} in terms of the employment rate and the average \backlog{} (recall that \texttt{Actual} does not incur over-allocation due to the definition of the capacity profile we chose for our case study). When compared with \texttt{Sampling}, for $\OverCost \geq 2$, the trajectory of outcome metrics for \texttt{RO-Learning} generally dominates that of \texttt{Sampling}. Specifically, for a given value of the employment outcome, \texttt{RO-Learning} achieves lower over-allocation and average \backlog{} compared to \texttt{Sampling}. This shows that the our learning-based approach better balances the three (potentially) conflicting outcome metrics. \SLedit{Indeed, The median improvement in the objective, as defined in Equation \eqref{ALG+obj} in \Cref{sec:model}, of \texttt{RO-Learning} over \texttt{Sampling} is 37\% for the year 2015 and 17\% for the year 2016. This improvement ranges from 3\% to 70\% across the considered range of cost parameters.}  \par
% range: min (improvement) ~ 3rd quantile of improvement | obj of the mindiscord is nonnegative

% \SLdelete{While we theoretically studied the setting where $\BuildUpCost$ can be quite large (e.g., on the order of $\sqrt{\TotalTime}$), we find that small values of $\BuildUpCost$ are sufficient to impact our algorithm in the real data of our partner agency. This is because the \backlog{} in our dataset can grow quite large due to the fact that (i) we do not reject any cases, and (ii) tied cases arrive in a non-stationary manner in our data set.}\SLcomment{I think we do not need to say this here (and it's confusing). So I'll just remove it.}

Finally, we note that even when $\BuildUpCost=0$, the average \backlog{} of \texttt{RO-Learning} is reasonably low compared to both the actual placement and \texttt{Sampling}. For example, focusing on the panel $\alpha=3$, the average \backlog{} of \texttt{RO-Learning} at $\BuildUpCost=0$ is roughly equivalent to that of \texttt{Sampling} at $\BuildUpCost=5$. As discussed in \Cref{sec:numerics}, this represents the inherent balancedness of the Learning-based approach. 

\begin{figure}[t]
  \begin{subfigure}{\linewidth}
    \centering
    \includegraphics[width=\linewidth]{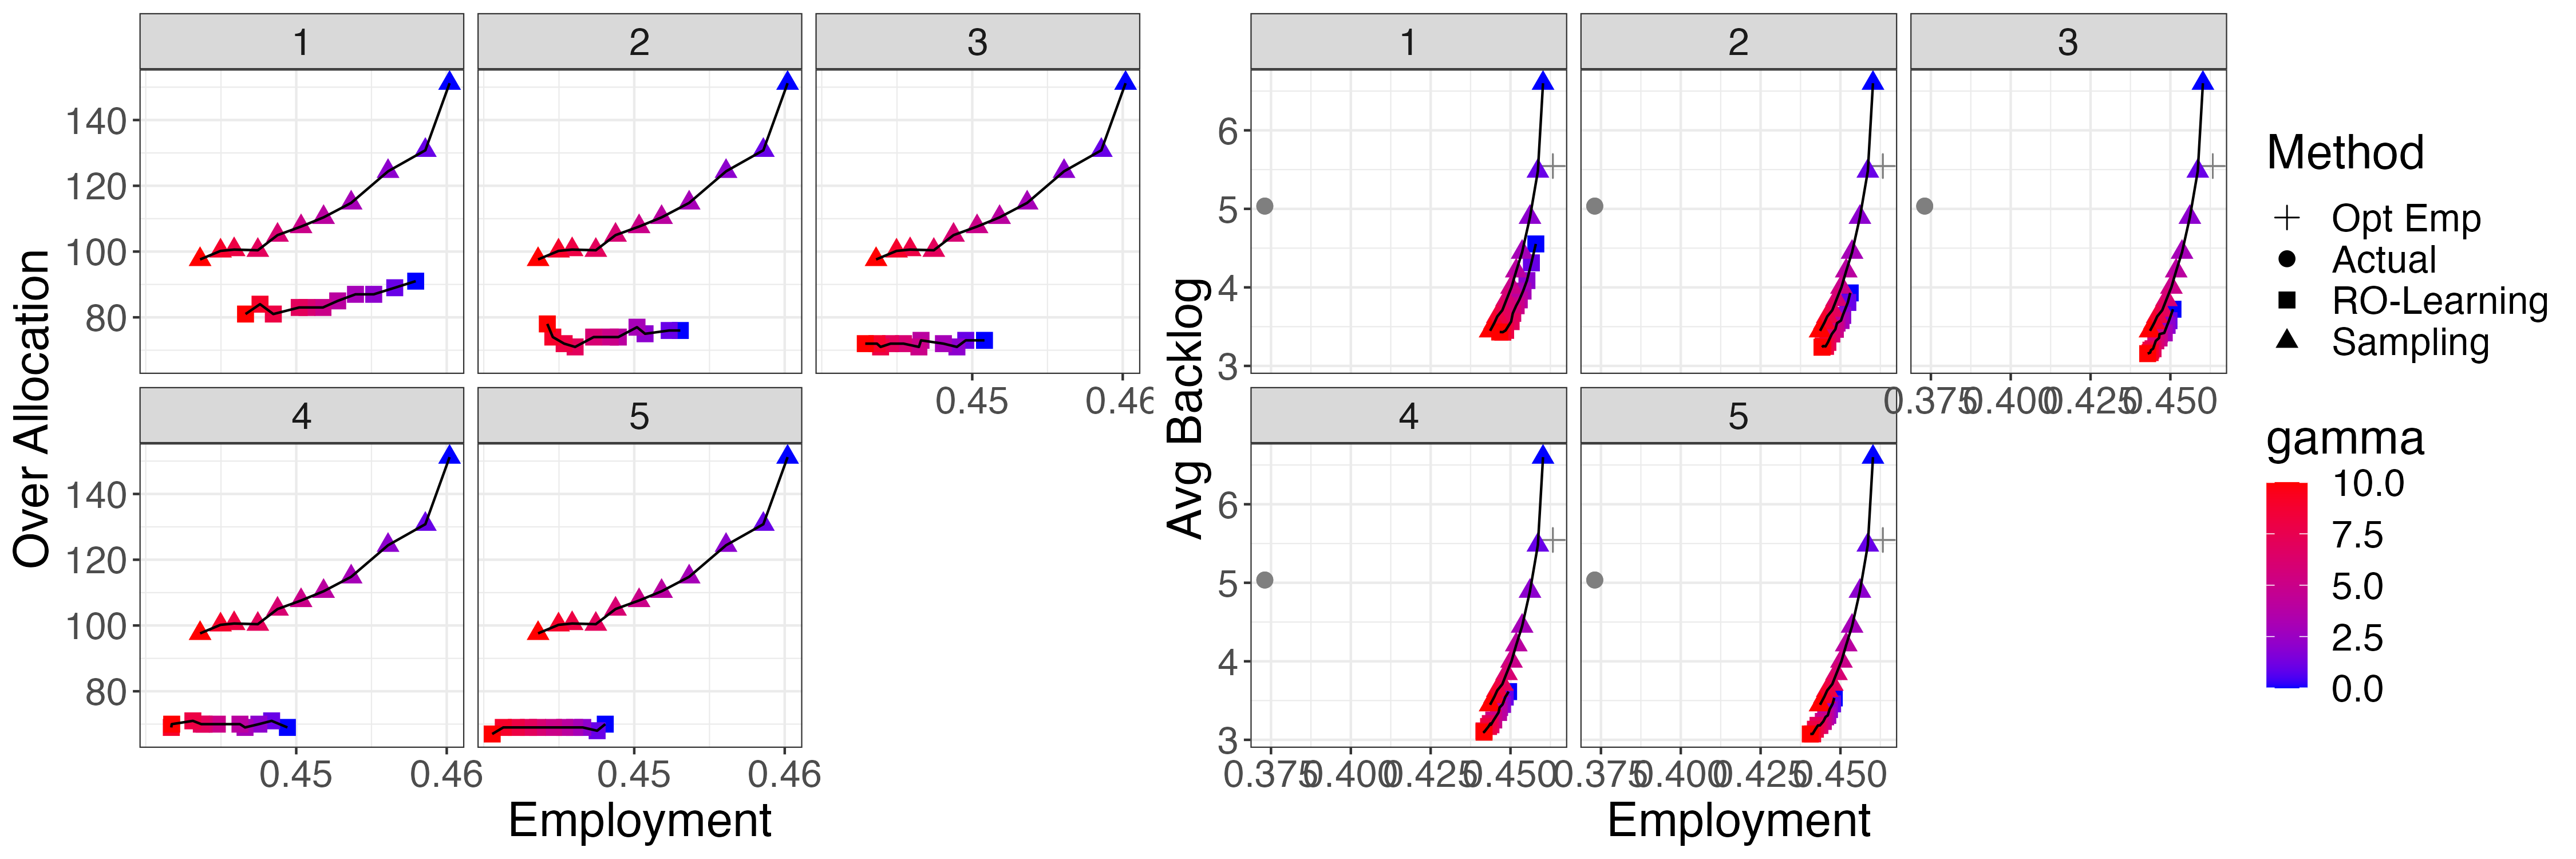}
    \caption{Year 2015}
    \label{fig:more+case:subfig1}
  \end{subfigure}

  \begin{subfigure}{\linewidth}
    \centering
    \includegraphics[width=\linewidth]{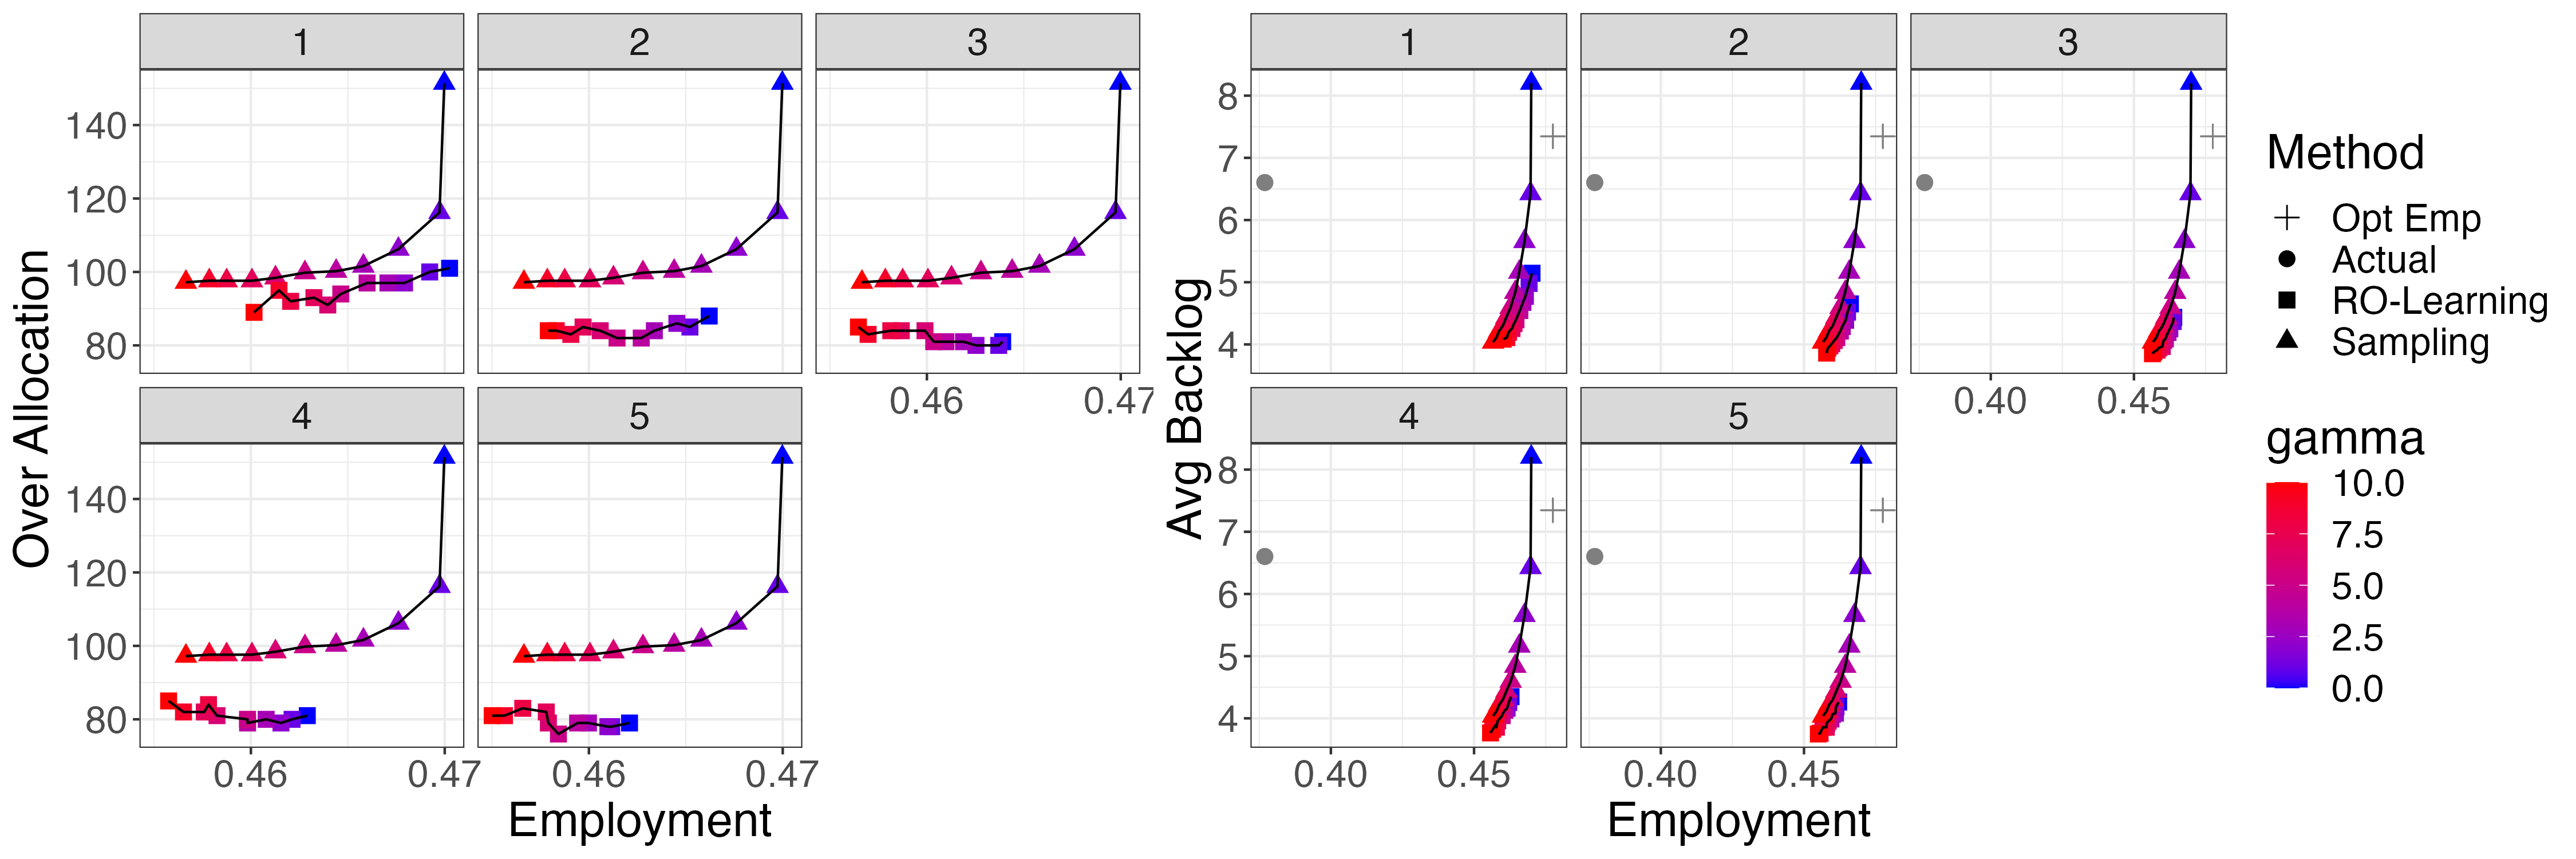}
    \caption{Year 2016}
    \label{fig:more+case:subfig2}
  \end{subfigure}

  \caption{Additional results for case Study with  $\boldsymbol{\OverCost \in \{1,2,..,5\}}$ and $\boldsymbol{\BuildUpCost \in \{0,1,...,10\}}$. 
  %Note: For \texttt{Sampling}, $\boldsymbol{\OverCost}$ is always equal to 1, and $\boldsymbol{\BuildUpCost}$ varies as shown. 
  In each panel, we display the trajectory of the outcome metrics of fixed $\boldsymbol{\OverCost}$ (label of the penal) and varying $\boldsymbol{\BuildUpCost}$.}
%  \SLcomment{EC Flagging: no boldsymbol for EC version. Turn it on for journal version. }
\SLcomment{\bf Figure for 2015 needs some fix}

%\SLcomment{questions/discussion on whether we want to say `we set $\OverCost=1$' or not is commented out (I think we can just remove it). @EP: please check whether behavior changes by yourself (see my responses commented out below) ---if seems to significantly change, we can discuss this again.}
%\EPcomment{I also added the comment that $\alpha=1$ for Sampling, but maybe we don't actually need to say this, since (I think?) Sampling would not change for $\alpha>1$.}
%\SLcomment{It should not change. In the absence of allocation balancing, we can prove that Sampling never over-allocates (in the program it solves at every time step) and therefore does not change its behavior with $\OverCost >1$. The same will be true as long as the difference of the 'adjusted' rewards in equation \eqref{eq:waiting+time} between two locations are at most $\OverCost$, which seems to be true in our simulation. I remember that when I checked numerically $\OverCost=1$ versus $\OverCost=3$ on the synthetic data (based on $\BuildUpCost=5$), the result did not change. If you want to test from your end, here's an efficient way of doing it by taking a deeper look at the result of $\OverCost=1$: for a fixed value of $\BuildUpCost$, if Sampling with $\OverCost=1$ did not over-allocate (with respect to $c_{t,i}$) at every time $\Timeidx$, then it means that the algorithm actually does not change its behavior for all values of $\OverCost \geq 1$. }
  \label{fig:more+case}
\end{figure}
