# Supplementary material for: Dynamic Matching with Post-allocation Service and its Application to Refugee Resettlement
Source: arXiv:2410.22992 source file (2025-07-02)
Supplement: Supplementary file 8 [file apx+over+allocation.tex]

{
\color{blue}
\subsection{Additional Results  of Over-allocation}\label{apx+over+additional}

In the U.S., affiliate-level capacities are determined through a collaborative process involving resettlement agencies, local affiliates, and the U.S. State Department. While resettlement agencies aim to adhere to these capacities, they are not enforced as hard constraints: affiliates are typically permitted to exceed their stated capacity by up to 10\% without additional approval~\citep{ahani2021placement}.\footnote{We also note that some degree of over-allocation is unavoidable due to the sequential arrival of tied cases.} Nevertheless, over-allocations are not costless. For example, since per-capita federal funding is largely associated with the approved capacity (see \Cref{footnote:over-allocation}), placements in excess of capacity may strain a resettlement agency’s financial resources. Our model captures these costs through a penalty term applied to each unit of over-allocation, reflecting the soft but costly nature of capacity constraints in practice.

However, not all over-allocation is equally costly. In particular, any matching that places an affiliate more than 10\% above its approved capacity must be formally approved by the State Department~\citep{dos2011coopagreement}, creating an additional administrative cost borne by the resettlement agency. For this reason, it is important to examine not only total over-allocation (aggregated across all affiliates, as reported in \Cref{sec:model}), but also how it is distributed—particularly whether, and to what extent, specific affiliates are “flagged” for exceeding the 10\% threshold.

To that end, Table~\ref{table:relative-overallocation} summarizes over-allocation outcomes at affiliates whose placements exceeded 110\% of their capacity. We use the same set of penalty parameters corresponding to \Cref{fig:performance}. The first column reports the number of such affiliates. While \texttt{RO-Learning} results in more flagged affiliates than \texttt{Sampling} in 2016 (5 vs.\ 3), most of these affiliates have small capacities. This is reflected in the next columns: the largest over-allocation among flagged affiliates under \texttt{RO-Learning} is only 7 cases, compared to 28 under \texttt{Sampling}. Finally, summing all placements beyond the 10\% threshold — each of which would have required formal reporting — \texttt{RO-Learning} yields a substantially lower total. Thus, the overall results indicate that \texttt{RO-Learning} not only incurs lower total over-allocation (as shown in \Cref{fig:performance} in \Cref{sec:numerics}), but also leads to a lower administrative burden associated with exceeding the 10\% threshold.

\begin{table}[htp]
    \centering
\caption{
Summary of over-allocation outcomes for flagged affiliates whose total placements exceeded 110\% of their capacity. Results correspond to penalty parameters $\boldsymbol{\alpha = 3}$ and $\boldsymbol{\gamma = 5}$ (as in \Cref{fig:performance}). 
Results are shown for 2015, with values in parentheses indicating outcomes for 2016.
}

    \label{table:relative-overallocation}
    \begin{tabular}{@{}lccc@{}}
        \toprule
        \textbf{Method} & 
        \makecell{\# Flagged Affiliates \\ with >{}10\% Over-allocation} & 
        \makecell{Max Absolute Over-allocation \\ Among Flagged Affiliates} & 
        \makecell{Total Over-allocation \\ Among Flagged Affiliates} \\
        \midrule
        \texttt{Sampling}      & 2 (3) & 34 (28) & 43.8 (46.0) \\
        \texttt{RO-Learning}   & 2 (5) & 29 (7)  & 35 (21)     \\
        \bottomrule
    \end{tabular}
\end{table}

}
