# Supplementary material for: Dynamic Matching with Post-allocation Service and its Application to Refugee Resettlement
Source: arXiv:2410.22992 source file (2025-07-02)
Supplement: Supplementary file 12 [file apx+fluid+proof.tex]

\subsubsection{Proof of \texorpdfstring{Claim \ref{fluid}}{}}\label{apx+fluid+pf}\par 
\SLcomment{Proof modified significantly. Double-check needed. We heavily rely on assumption that $\sum_{\Locidx=1}^m \CapRatio_\Locidx = 1 $ (or $\geq 1$).}

\SLedit{Consider the following optimization problem.}
\begin{equation}
\begin{split}
% 2nd line
%\SinglePrimal(\OverCost)
\SLedit{\SinglePrimal_{\mathcal{Z}}}&:= \max_{\substack{\DecisionVec(\Arrival) \in \FeasibleSet{\Target} \\
\forall \Arrival \in \ArrivalSupp}} \E[\Weightvec\cdot \DecisionVec(\Arrival)] \quad \text{s.t.} \ 
    % constraint
%\E\left[\Indicator[\Target=0]\cdot\DecisionVec(\Arrival)\right] \leq \CapRatioVec  \label{eq:P} 
\E\left[\DecisionVec(\Arrival)\right] \leq \CapRatioVec  \label{eq:P}
\end{split}
\end{equation}
where the expectation is with respect to $\mathbf{A} = (\Weightvec, \Target)\sim \ArrivalDist$. This optimization problem can be viewed as the stochastic program maximizing the expected per-period net \allocation{} reward. The decision is to choose a function (control) $\DecisionVec: \ArrivalSupp \to \Simplex$ subject to $\DecisionVec(\Arrival) \in \FeasibleSet{\Target}
$. That is, for each arrival type $\Arrival = (\Weightvec, \Target)$, we choose the matching rate $\DecisionVec(\Arrival) \in \Simplex$ if $\Target = 0$ (free case) or we set it as $\DecisionVec(\Arrival) = \BasisVec{\Target}$ otherwise. The objective is to maximize the functional $\E[\Weightvec\cdot\DecisionVec(\Arrival)]$, which is the expected per-period \allocation{} reward given the control $\DecisionVec(\cdot)$, subject to \SLedit{the (ex-ante) capacity constraint on the matching rate}. \SLedit{Note that, due to our assumption that $\CapRatio_\Locidx \geq \P[\Target=\Locidx]$, the program is always feasible and therefore $\mathcal{P}_{\mathcal{Z}}$ is well-defined. }

Define $\bar{\DecisionVec}(\cdot)$ as the optimal mapping that solves the single-period primal problem in \eqref{eq:P}. In the following, we show that $\bar{\DecisionVec}(\cdot)$ satisfies the condition \ref{fluid:feasible}-\ref{fluid:opt} stated in Claim \ref{fluid}.\par 
%%%%%%%%%%%%%%%%%%%%%%%%%%
\noindent{\bf Proof of Claim \ref{fluid} and \ref{fluid:feasible}-\ref{fluid:rate}.} This directly follows from the feasibility condition of the mapping $\bar{\DecisionVec}(\cdot)$. \hfill\halmos \par

\noindent{\bf \bf Proof of Claim \ref{fluid}-\ref{fluid:opt}.} Let $\{\hat{\DecisionVec}_\Timeidx\}_{\Timeidx=1}^\TotalTime$ be an arbitrary feasible \allocation{} profile. That is, it satisfies
\begin{align*}
 % Type feasibility 
    \hat{\DecisionVec}_\Timeidx &\in \FeasibleSet{\Target_\Timeidx} \quad \forall \Timeidx \in [\TotalTime] \\ 
    \sum_{\tau=1}^\Timeidx \Indicator[\Target_\tau = 0] \Decision_{\tau,\Locidx} 
    &\leq \left(\Capacity_\Locidx - \sum_{\tau=1}^\Timeidx \Indicator[\Target_\tau = \Locidx]\Decision_{\tau,\Locidx}\right)_{+} \quad \forall \Timeidx \in [\TotalTime], \Locidx \in [\Locnum].
\end{align*}

It suffices to prove
\[
%\SinglePrimal(\OverCost)
\SinglePrimal_{\mathcal{Z}}
\geq 
\E\Big[
\frac{\NetReward({\{\hat{\DecisionVec}_\Timeidx\}}_{\Timeidx=1}^\TotalTime; \OverCost)}{\TotalTime}
\Big].
\]

To prove this, we make some observations. For given target affiliate $\Target \in \{0\}\cup[m]$, we first define a correspondence ${\mathcal{Y}}(\cdot)$ such that
\begin{equation}
    {\mathcal{Y}}(\Target) = \begin{cases}
    \Delta_m \quad \text{if $\Target=0$} \\
    \{\DecisionVec\in \R_+^m: \Decision_\Locidx \leq \Indicator[\Target=\Locidx], \ \forall \Locidx \in [\Locnum]\} \quad \text{otherwise.}
    \end{cases}
\end{equation}
Unlike our original feasibility set $\mathcal{Z}(\cdot)$, ${\mathcal{Y}}(\cdot)$ allows for inaction for tied cases (as well as for free cases). Define a static control (analogous to \eqref{eq:P}) as 
\begin{equation}
\SinglePrimal_{\mathcal{Y}}:= \max_{\substack{\DecisionVec(\Arrival) \in \mathcal{Y}(\Target) \\
\forall \Arrival \in \ArrivalSupp}} \E[\Weightvec\cdot \DecisionVec(\Arrival)] \quad \text{s.t.} \ 
    % constraint
%\E\left[\Indicator[\Target=0]\cdot\DecisionVec(\Arrival)\right] \leq \CapRatioVec  \label{eq:P} 
\E\left[\DecisionVec(\Arrival)\right] \leq \CapRatioVec   
\end{equation}
\SLedit{We first note that, under our assumption $\sum_{\Locidx=1}^\Locnum \CapRatio_\Locidx = 1$, we must have $\SinglePrimal_\mathcal{Z} = \SinglePrimal_{\mathcal{Y}}$ because, in expectation, accepting every case (i.e. $\E[z(\Arrival)] = \CapRatioVec$) is feasible and the reward is non-negative.} 

We now define a related dual problem to each of $\SinglePrimal_\mathcal{Z}$ and $\SinglePrimal_\mathcal{Y}$ as 
\begin{equation}
  \textsf{D}_{\mathcal{Z}}(\boldsymbol{\phi}):= \E\left[
\max_{\DecisionVec(\Arrival) \in \FeasibleSet{\Target}}(\Weightvec - \boldsymbol{\phi})\cdot \DecisionVec(\Arrival) + \CapRatioVec\cdot \boldsymbol{\phi}
    \right], \quad 
% definition of D*
\SingleDual_{\mathcal{Z}} := \min_{\boldsymbol{\phi}\geq \mathbf{0}} \textsf{D}(\boldsymbol{\phi}).  
\end{equation}
\begin{equation}
  \textsf{D}_{\mathcal{Y}}(\boldsymbol{\phi}):= \E\left[
\max_{\DecisionVec(\Arrival) \in \mathcal{Y}(\Target)}(\Weightvec - \boldsymbol{\phi})\cdot \DecisionVec(\Arrival) + \CapRatioVec\cdot \boldsymbol{\phi}
    \right], \quad 
% definition of D*
\SingleDual_{\mathcal{Y}} := \min_{\boldsymbol{\phi}\geq \mathbf{0}} \textsf{D}(\boldsymbol{\phi}).  
\end{equation}

By the compactness and convexity of $\FeasibleSet{\Target}$ and $\mathcal{Y}(\Target)$ for all $\Target \in \{0\}\cup[m]$, a straightforward application of Sion's minmax theorem \citep{sion1958general} implies that $\SingleDual_{\mathcal{Z}} = \SinglePrimal_{\mathcal{Z}}$ and $\SingleDual_{\mathcal{Y}} = \SinglePrimal_{\mathcal{Y}}$. Because $\SinglePrimal_{\mathcal{Z}} = \SinglePrimal_{\mathcal{Y}}$, we further have $\SingleDual_{\mathcal{Z}} = \SingleDual_{\mathcal{Y}}$.

Given these ingredients, we show that, for any feasible \allocation{} profile ${\{\hat{\DecisionVec}_\Timeidx\}}_{\Timeidx=1}^\TotalTime$, that $\SinglePrimal_{\mathcal{Z}}\geq \E[\frac{\NetReward(\{\hat{\DecisionVec}_\Timeidx\}_{\Timeidx=1}^\TotalTime; \OverCost)]}{\TotalTime}$ in the following. 
\begin{comment}
Let $N_{\TotalTime,\Locidx} := \sum_{\Timeidx=1}^\TotalTime \Indicator[\Target_\Timeidx=\Locidx]$ and event $G_\TotalTime$ as $
    G_\TotalTime := \left\{ N_{\Timeidx, \Locidx} \leq \Capacity_\Locidx, \forall \Locidx \in [\Locnum]\right\}$. Note that $\Indicator[\Target_\Timeidx = \Locidx]$ is an i.i.d. binary random variable and with $\tau_\Locidx := \P[\Target_\Timeidx = \Locidx] < \rho_\Locidx$. By a straightforward application of Hoeffding's inequality and union bound, we have that $\P[G_\TotalTime] \geq 1-\sum_{\Locidx=1}^\Locnum \exp(-2(\CapRatio_\Locidx - \tau_\Locidx)^2 ) = 1 - \BigO(1/\TotalTime^2)$ where the last equality follows from our assumption that $\CapRatio_\Locidx - \tau_\Locidx = \Theta(1)$. Hence, we have
\end{comment}
% test:
\begin{align}
%first line: original problem with Z, and dynamic capacity
%%%%%%%%%%%%%%%%%%%%%%%%%%%%%%%%%%%
&\E[\NetReward(\{\hat{\DecisionVec}_\Timeidx\}_{\Timeidx=1}^\TotalTime; \OverCost)] \nonumber  \\
&\leq \E\left[\max_{\DecisionVec_\Timeidx \in \FeasibleSet{\Target_\Timeidx}, \Timeidx\in [\TotalTime]}
% reward
\sum_{\Timeidx=1}^\TotalTime
\Weightvec_\Timeidx \cdot \DecisionVec_\Timeidx
    % over-allocation
    - \OverCost\sum_{\Locidx=1}^{\Locnum} \PositivePart{\sum_{\Timeidx=1}^\TotalTime \DecisionEach - \Capacity_\Locidx } \quad 
    % constraint 
    \text{s.t}\    \sum_{\tau=1}^\Timeidx \Indicator[\Target_\tau = 0] \Decision_{\tau,\Locidx} 
    \leq \left(\Capacity_\Locidx - \sum_{\tau=1}^\Timeidx \Indicator[\Target_\tau = \Locidx]\Decision_{\tau,\Locidx}\right)_{+} \quad \forall \Timeidx \in [\TotalTime], \Locidx \in [\Locnum]\right] \label{ineq:upper+z+hat}\\
%%%%%%%%%%%%%%%%%%%%%%%%%%%%%%%%%%%%
% second line: relax Z to Y 
&\leq \E\left[\max_{\DecisionVec_\Timeidx \in \mathcal{Y}(\Target_\Timeidx), \Timeidx\in [\TotalTime]}
% reward
\sum_{\Timeidx=1}^\TotalTime
\Weightvec_\Timeidx \cdot \DecisionVec_\Timeidx
    % over-allocation
    - \OverCost\sum_{\Locidx=1}^{\Locnum} \PositivePart{\sum_{\Timeidx=1}^\TotalTime \DecisionEach - \Capacity_\Locidx } \quad 
    % constraint 
    \text{s.t}\  \sum_{\tau=1}^\Timeidx \Indicator[\Target_\tau = 0] \Decision_{\tau,\Locidx} 
    \leq \left(\Capacity_\Locidx - \sum_{\tau=1}^\Timeidx \Indicator[\Target_\tau = \Locidx]\Decision_{\tau,\Locidx}\right)_{+} \quad \forall \Timeidx \in [\TotalTime], \Locidx \in [\Locnum]\right]
    \label{line:relax+Y}
    \\
%%%%%%%%%%%%%%%%%%%%%%%%%%%%%%%%
% 3rd line : relax capacity constraint
&\leq \E\left[\max_{\DecisionVec_\Timeidx \in \mathcal{Y}(\Target_\Timeidx), \Timeidx\in [\TotalTime]}
% reward
\sum_{\Timeidx=1}^\TotalTime
\Weightvec_\Timeidx \cdot \DecisionVec_\Timeidx
    % over-allocation
    - \OverCost\sum_{\Locidx=1}^{\Locnum} \PositivePart{\sum_{\Timeidx=1}^\TotalTime \DecisionEach - \Capacity_\Locidx } \quad 
    % constraint 
    \text{s.t}\ \sum_{\Timeidx=1}^\TotalTime \Indicator [\Target_\Timeidx  = 0]\DecisionEach \leq \left(\Capacity_\Locidx - \sum_{\Timeidx=1}^\TotalTime \Indicator[\Target_\Timeidx = \Locidx]\Decision_{\Timeidx,\Locidx} \right)_{+}, \forall \Locidx \in [\Locnum]\right] 
    \label{line:relax+cap}\\
%%%%%%%%%%%%%%%%%%%%%%%%%%%%%%%%%%%%%
% 4th: at optimum, we don't want to set \sum_{\tau=1}^\Total > c_i because \alpha>1
&= \E\left[\max_{\DecisionVec_\Timeidx \in \mathcal{Y}(\Target_\Timeidx), \Timeidx\in [\TotalTime]}
% reward
\sum_{\Timeidx=1}^\TotalTime
\Weightvec_\Timeidx \cdot \DecisionVec_\Timeidx
    % over-allocation
    %-\OverCost\sum_{\Locidx=1}^{\Locnum} \PositivePart{\sum_{\Timeidx=1}^\TotalTime \DecisionEach - \Capacity_\Locidx } 
    \quad 
    % constraint 
    \text{s.t}\ \sum_{\Timeidx=1}^\TotalTime \DecisionEach \leq \Capacity_\Locidx, \forall \Locidx \in [\Locnum]\right] 
    \label{line:no+over+Y}\\
%%%%%%%%%%%%%%%%%%%%%%%%%%%%%%%%%%%
% 5th: Lagrangicy
&\leq \E\left[
% begin bracket
%\left(
\max_{\DecisionVec_\Timeidx\in \mathcal{Y}(\Target_\Timeidx), \Timeidx\in [\TotalTime]}
\sum_{\Timeidx=1}^{\TotalTime}
    % reward 
    \Weightvec_\Timeidx \cdot \DecisionVec_\Timeidx
% no over-allocation
    % relaxed cap constraint  
- \boldsymbol{\phi}\cdot\left(\sum_{\Timeidx=1}^\TotalTime  \DecisionVec_\Timeidx -\CapacityVec 
\right)
% \end bracket
%\right
%)
% indicator
%\cdot \Indicator[G_\TotalTime]
    \right]
% 
%+ \BigO(1/\TotalTime)
% for all phi    
\quad \forall \boldsymbol{\phi}\geq\mathbf{0}
\label{line:lagragify}
\\
%%%%%%%%%%%%%%%%%%%%%%%%%%%%%%%%%%
% 6th: simplify 
&=
\E\left[ 
%\start bracket
\sum_{\Timeidx=1}^\TotalTime
\max_{\DecisionVec_\Timeidx \in \mathcal{Y}(\Target_\Timeidx)}\{
(\Weightvec_\Timeidx - \boldsymbol{\phi})\cdot \DecisionVec_\Timeidx
+ \boldsymbol{\phi}\cdot \CapRatioVec
\}
%\end bracket
% indicator
\right]
% for all phi
\quad \forall \boldsymbol{\phi}\geq \mathbf{0} \label{line:separable}\\ 
%%%%%%%%%%%%%%%%%%%%%%%%%%%%%%%%%%%
%%%%%%%%%%%%%%%%%%%%%%%%%%%%%%%
% 7th: iid 
&= \TotalTime \textsf{D}_{\mathcal{Y}}(\boldsymbol{\phi}) \quad \forall \boldsymbol{\phi}\geq \mathbf{0}
\label{line:iid}
%%%%%%%%%%%%%%%%%%%%%%%%%%%%%%%%%%%%
\end{align}
% 2nd: relax+Y
In line \eqref{line:relax+Y}, we used the fact that $\mathcal{Z}(\Target_\Timeidx) \subseteq \mathcal{Y}(\Target_\Timeidx)$ for all $\Timeidx \in [\TotalTime]$, and hence relaxing the feasibility set can only increase the maximum net matching reward.
% 3rd: relax+cap 
Line \eqref{line:relax+cap} follows from relaxing the capacity constraint (i.e., imposing the capacity constraint at only last period $\TotalTime$). 
% 4rd
To understand line \eqref{line:no+over+Y}, we first note that, because $\OverCost>1$ and $w_{\Timeidx,\Locidx} \leq 1$ by our assumption, the optimal solution of the maximization problem in line \eqref{line:relax+cap} must satisfy $\sum_{\Timeidx=1}^\TotalTime \Indicator[\Target_{\Timeidx=i}]\Decision_{\Timeidx,\Locidx} \leq \Capacity_\Locidx$ for all $\Locidx \in [\Locnum]$: otherwise, we can always drop a tied case and strictly increase the net matching reward (we emphasize that this is only true when type-feasibility set is $\mathcal{Y}(\cdot)$). As such, the capacity constraint in line \eqref{line:relax+cap} reduces to $\sum_{\Timeidx=1}^\TotalTime \Decision_{\Timeidx, \Locidx}\leq \Capacity_\Locidx$ for all $\Locidx \in [\Locnum]$ and hence \eqref{line:no+over+Y} follows.\footnote{Note that $z_{\Timeidx, \Locidx} = (\Indicator[\Target_\Timeidx=0] + \Indicator[\Target_\Timeidx=1])z_{\Timeidx,\Locidx}$ by definition of $\mathcal{Y}$.}
%5-6th
Lines \eqref{line:lagragify} follows by a standard Lagrangification of the capacity constraint of the optimization problem in line \eqref{line:no+over+Y}.
%7th: line i.i.d.
Finally, line \eqref{line:iid} is because
the arrival type $\Arrival_\Timeidx = (\Weightvec_\Timeidx, \Target_\Timeidx)$ is i.i.d. random variables. \par 
By taking minimum over $\boldsymbol{\phi} \geq \mathbf{0}$ on line \eqref{line:iid}, we conclude that
\begin{equation}
\E[\NetReward(\{\hat{\DecisionVec}_\Timeidx\}_{\Timeidx=1}^\TotalTime; \OverCost)] \leq \TotalTime \SingleDual_{\mathcal{Y}}.
\end{equation}
The proof is completing by noting that $\SingleDual_{\mathcal{Y}} = \SingleDual_{\mathcal{Z}} = \SinglePrimal_{\mathcal{Y}}$
. \hfill \halmos
