# Supplementary material for: Dynamic Matching with Post-allocation Service and its Application to Refugee Resettlement
Source: arXiv:2410.22992 source file (2025-07-02)
Supplement: Supplementary file 13 [file EC+response.tex]

\section{Overview of Changes/Additions Based on EC Reviews}\label{apx+ec+response}
We are thankful to the EC review team for their support for our paper, and for the great and constructive
comments that helped us improve our work. We have substantially revised the paper to address their comments. For ease of reference, in this section we first include the EC reviews in \Cref{subsec:ec+reviews}. Then, we provide
an overview of the most significant changes/additions in \Cref{subsec:ec+responses}.

\subsection{EC reviews}\label{subsec:ec+reviews}

% Meta review
\noindent{\bf Meta Review:} 
{\itshape All reviewers appreciated this paper. In particular, the problem is clearly very important, and the theoretical contribution is substantial with several new features (such as distribution-free algorithms and dynamic capacity). The review team also thought that the paper was clearly written, although some issues were raised, and we hope you can incorporate the comments in the final version.

The rebuttal also helped clarify some issues, and the announcement that you can deal with multiple knapsack constraints is appreciated. The recommendation is thus to ACCEPT the paper.}

\medskip

% EC Review 1
\noindent{\bf EC Review A:}
{\itshape
Motivated by refugee resettlement process in the U.S., this paper studies a dynamic matching problem with a novel aspect (called post-allocation service). The authors study a finite-horizon discrete-time model, where one refugee case arrives at each time period. The case is either tied (must be matched to a target affiliate) or free to be matched to any affiliate. Each affiliate has a known fixed capacity, where each match consumes one capacity. There are $m$ affiliates and $T$ cases. After each match is performed (where the platform commits to each match), each affiliate is associated with a server whose availability is random with a known service rate. The server is called congested if there are matched cases waiting to get a service. The problem has the following penalty costs: if an affiliate is over-allocated (the total number of matched cases exceeds the capacity), then we pay $\alpha$ for each unit of over allocation. If the server is congested, we pay $\gamma$ for each unit of the time average backlog. The goal is to maximize the total collected reward minus penalty costs over T periods in expectation. The authors study a natural performance metric (regret), where regret  is the worst possible difference between the offline benchmark's performance (full information on sequence of arrivals and service availability) and the online policy's performance. 

The authors first provide a lower bound on achievable regret. Then the authors exploit the knowledge on the dual variables of the offline benchmark to devise their algorithm (called Congestion-Aware Dual-Learning). Under certain regimes, they prove that the algorithm achieves sub-linear regret. The key assumption here is that we have full information on the backlog of servers. The authors also devise an algorithm under the assumption that this information is unknown, which also achieves sub-linear regret. Finally, the authors run simulations to compare the performances of the proposed policies.

\medskip

Strengths and Weaknesses:
\begin{itemize}
    \item Strengths: The study is motivated by a very important problem. Overall the paper is well written.
    \item Weaknesses: Certain proofs are hard to follow in the main body and lack intuitive explanations. Same goes for Definition 2.1, where it is not clear in the beginning why do we consider these two regimes in terms of $\epsilon$.
\end{itemize}

\medskip

Comments: 
%Questions for Author Response
%-----------------------------
\begin{enumerate}
    \item I am still lacking motivation for the fact that the purpose is to find algorithms that do not rely on distributional knowledge. Can you elaborate more on the observed fluctuations in the arrivals?
    \item Do we know anything about maximizing the dual-adjusted scores without time invariance assumptions on ($\boldsymbol{\theta}^*, \boldsymbol{\lambda}^*)$ and the stationarity of arrivals and services (regarding Proposition 3.1)? Motivated from the argument that there is observed fluctuations in the composition of refugee pools across the years, this seems important.  
    \item  Can you elaborate more around Definition 2.1 on the importance of these two regimes?
\end{enumerate}
}

\medskip

%%%%%%%%%%%%%%%%%%%%%%%%%%%%%%%%%%%%%%%%%%%%%%%%%%%%%%%%%%%%%%
% EC Review 2
\noindent{\bf EC Review B:}
{\itshape
The paper investigates a dynamic matching+queuing model motivated by the problem of resettling refugees in the United States. The model can be seen as the concatenation of two parts. The first part is a fairly standard online two-sided matching problem where one side (cities where the refugees can be resettled, called ``affiliates" in the model) has integer capacities, while the other (refugees) has capacity 1, come in an online fashion as i.i.d. realizations to an unknown underlying distribution, and need to be matched immediately. The allocation of refugee t to affiliate $i$ consumes one unit of $i$'s capacity and gives a profit $w_{t,i}$ (an additional, yet apparently not too relevant constraints is given by some refugees that must be matched to specific affiliates). The second part is a ``dynamic queuing model" where each affiliate $i$ acts as a server with a certain service rate, and each refugee assigned to $i$ in the first part joins the server's queue (one should think of this second part as refugees needing post-assignment support like translations, help in job search, etc.). The goal is to maximize the expect profit of the matching minus a penalty for exceeding the capacities of the affiliates, and for the backlog, which is a function of the length of the queues. 

The algorithms proposed use classical scoring techniques based on dual variables to a certain convex program, but with a twist given by the ``dynamic queuing model", which requires the addition of time-dependent dual variables with respect to the static ones. The first algorithm proposed, CA-DL, achieves sublinear regret with respect to the offline optimum that has full clairvoyance with respect to the realizations of the distributions. A modification of CA-DL, dubbed CO-DL, that takes decisions ignoring information on the current backlog, also achieves sublinear regrets in many regimes. The algorithms are then applied to data from a partner resettling agency, showing improvement with respect to competing methods.

\medskip

Strengths and Weaknesses:
\begin{itemize}
    \item  The paper investigates an original twist on the classical online matching problem. The algorithms have a number of non-trivial moving parts, although I was not able to find a fundamental new idea (if such an idea is present, I suggest the authors to highlight it). The technical analysis appear to be non-trivial. The application is interesting and theoretical results are support by numerical experiments.
\end{itemize}


\medskip

Comments: 
\begin{enumerate}
    \item In many refugee resettlement models, affiliates have one or more knapsack constraints, and each refugee can consume multiple units of each resource. Your model can be easily extended to this case. Can your algorithms be adapted to this scenario and how do they perform?
\end{enumerate}
%Questions for Author Response
%-----------------------------
}

\medskip

% EC Review 3 
\noindent{\bf EC Review C:}
{\itshape
The paper studies the assignment of refugees to local organizations in the US. Resettlement agencies have to assign refugees to their \textit{affiliates}. The problem has been studied from various perspectives in both the CS and econ literatures. There are two key new aspects in this paper. First, the proposed algorithms do not rely on previous data. Second, the model and the algorithms incorporate a dynamic resource (e.g., translators) that refugees will need after they are resettled. The authors simulate their algorithms using data from a resettlement agency and show that they provide good results in an uncertain environment (over both the future arrival of refugees and the availability of the dynamic resource).

\medskip

Strengths and Weaknesses:
\begin{itemize}
\item (+) The paper combines a strong theoretical contribution with a strong applied contribution.

\item (+) On the theory side, new aspects are introduced; in particular, the fact that the algorithm does not rely on previous data and the introduction of a dynamic capacity constraint (in addition to the static one).

\item (+) On the applied front, the algorithms provided are directly relevant to US resettlement agencies (and with some modifications could be useful in other countries too). The number of resettled refugees in the US can change drastically from one year to the next so the ability not to rely on past data is valuable.

\item (+) The paper is extremely well-written.

\item (-) The value of not relying on previous data is very well-motivated. The importance of the post-allocation service is less clear to me (see first question to the authors).
\end{itemize}

\medskip

Comments: 

I'm mainly asking the following questions because I'm curious, but perhaps reflecting on them can help with the motivation of the paper.
\begin{enumerate}
    \item How important is the post-allocation service? My understanding is that the key constraint is the number of people assigned to an affiliate (as these numbers are agreed with the State Department) but that there's flexibility when it comes to other services. Are you adding this mainly as a theoretical exercise, or is there a strong push from the agency with which you're working to take this into account?
    \item Your model assigns one refugee (or family) at a time. Typically, agencies match multiple families to affiliates at a time. Would this have an impact or is there no loss in just taking those families one by one?
    \item You mention that your model and algorithm can be trivially extended to families having more than one member (and therefore taking multiple units of capacity). Would this still be the case if multiple families were matched at once or would this start causing problems?
\end{enumerate}
}


\smallskip

%%%%%%%%%%%%%%%%%%%%%%%%%%%%%%%%%%%%%%%%%%%%%%%%%%%%%%%
%\SLcomment{Regarding your quesiton on whether we want to mention we moved the additional case study from the appendix to the main body, I don't think we need to mention it here. To me it does not seem to add too much value.}
\subsection{Summary of Changes}\label{subsec:ec+responses}
Based on the thoughtful comments we received (listed above), we have made substantial changes and additions to our paper. Our changes include:\footnote{
In addition to the outlined changes, we slightly modified the capacity constraint (see inequality \eqref{hard+constraint:t} $\forall t \in [\TotalTime]$ in \Cref{sec:model}) and our algorithms accordingly. In essence, this new capacity constraint ensures that no over-allocation can occur from free cases. This constraint is stricter than the one in the EC version and it is both more natural and aligned with our partner's practices. } 
%\SLcomment{Let's think of a better ordering. }
\begin{itemize}
% part 1
    \item {\bf Generalizing Theoretical Development to Multiple Resource Types.} In response to EC Review B and Meta review, we have added \Cref{apx+non+unit+size} \ECedit{(along with \Cref{footnote:multiple+knapsack})}, where we study a more general setting in which each case may require multiple types of resources (each with its own capacity constraint) and may consume more than one unit of capacity. In particular:
    \begin{enumerate}[label=(\alph*)]
        \item In \Cref{subsec:generalized+model}, we describe how to generalize our modeling framework. Then, in \Cref{subsec+generalized+algos}, we describe how to generalize our algorithms and their analysis, mainly focusing on \CA{} (\Cref{ALG+Surrogate+D}) for brevity.
        \item In a nutshell, we show that under the natural assumptions of having a constant number of types and a constant bound on the maximum number of capacity units that each case can consume, our regret bounds remain the same in terms of scaling with $\TotalTime$ (see \Cref{cor:CA+new} and its related discussion).
    \end{enumerate}

%%%%%%%%%%%%%%%%%%%%%%%%%%%%%%%%5
% part 2 
    \item {\bf Expanding Case Study to Batched Arrivals.} In response to EC Review C, in the newly added  \Cref{apx+batching} (along with \Cref{footnote:batching}), we investigate the impact of batched arrivals in the context of our case study. In particular:%\ECcomment{I added footnote \ref{footnote:batching} when we describe our model in \Cref{subsec:intro+contribution} to mention this appendix in the main paper.} 
    \begin{enumerate}[label=
    (\alph*)]
    \item In \Cref{apx+batching+model}, we describe how to modify our framework for batched arrivals. Then in \Cref{subsubsec:naive} and \Cref{apx+batch+b+iterate}, we present two modifications of \texttt{RO-Learning} (our base algorithm presented in \Cref{sec:numerics}) to account for batched arrivals. In  \Cref{table:performance+batch}, we compare the performance of our base algorithm (which ignores batched arrivals) to these modifications. 
    \item This exercise suggests that incorporating batched arrivals in the setting of our case study may offer a small performance improvement (by 3\% in terms of the objective value defined in equation \eqref{ALG+obj}). However, achieving this gain requires a considerably more complex and less interpretable algorithm. Further, such additional complexity appears necessary for performance improvement: as discussed in \Cref{subsubsec:naive}, a naive modification of \texttt{RO-Learning} indeed hurts performance. Therefore, it is unclear whether the small performance gain from leveraging batched arrivals outweighs the additional complexities.
    \end{enumerate}
%%%%%%%%%%%%%%%%%%%%%%%%%%%%%%%
% part 3
\item{{\bf Elaboration on Modeling Choices.}} Based on numerous great comments made from the EC review team, we have added clarifications in various sections to further elaborate on our modeling choices. In particular:
    \begin{enumerate}[label=
    (\alph*)]
        \item In response to EC Review A, we have added \Cref{apx+within+year+variations} (along with \Cref{footnote:within+year+variation} in \Cref{subsec:intro+background}) to further elaborate on the distinction between within-year and across-years variation as well as {the motivation for taking a distribution-free approach to algorithm design in this application (as acknowledge by Reviwer C)}. Further, in \Cref{subsec:intro+background} (in the fourth paragraph) and \Cref{apx+within+year+variations} (in the first paragraph), we clarified that the decision-making horizon for refugee resettlement is one year in light of the annual quota. %\ECcomment{I added  Footnote \ref{footnote:within+year+variation} to this appendix in the main paper. }
        \item In response to Reviwer C, in \Cref{subsec:intro+background} (in the fourth paragraph) and \Cref{subsec:data} (in the penultimate paragraph), 
        we have further elaborated on the importance of post-allocation service and smooth matching for our partner agency. Furthermore, in \Cref{footnote+post+allocation+service}, we emphasize that managing congestion in post-allocation service and adhering to annual quotas are different goals, both of which are captured in our objective function (equation \eqref{ALG+obj}).
        \item To address Reviewer A's comment, following \Cref{def:eps+regimes}, we explained our motivation for the two distinct regimes regarding $\epsilon$ (by borrowing an analogy from queueing literature). Specifically, we highlighted that treating these regimes separately reveals distinct performance of our algorithms, as shown in \Cref{sec:alg+design} and \Cref{subsec:alg+surrogate+primal}.
    \end{enumerate}
\item{{\bf Highlighting Technical Aspects.}} To address thoughtful comments made by the EC review team, we have added clarifications and elaborations in various sections to highlight our technical contribution as well as provide more intuitive explanation of our proofs. In particular:
    \begin{enumerate}[label=
    (\alph*)]
    \item We have significantly expanded our discussion of the related literature in \Cref{subsec:lit+review} with an emphasis in highlighting the fundamental technical differences between our framework and previous work on (i) online resource allocation (in the sixth paragraph of \Cref{subsec:lit+review} starting with ``\emph{Closest to our work ...}") and (ii) matching queues (in the last two paragraphs of \Cref{subsec:lit+review}). While expanding the literature review, we also highlighted how we addressed these novel technical challenges of our framework. Furthermore, we have also added \Cref{apx:lyapunov} to elaborate on a connection between the design of our first algorithm (\Cref{ALG+Surrogate+D}) and Lyapunov optimization. 
    % remove the items below
    %\item In response to Reviwer B's comment, given that we had provided a short version of literature review in the EC version (due to space limitation), we have significantly expanded the literature review in \Cref{subsec:lit+review} to better highlight our technical contribution. Specifically, in the seventh paragraph of \Cref{subsec:lit+review}, we emphasized that, while we draw on classical scoring techniques in online resource allocation, the time-varying nature of dual variables (\Cref{prop:offline}) deviates from the literature. Consequently, we introduce several innovative ideas including (i) novel combination of adversarial learning and drift analysis to design and analyze \CA{} (we have also added \Cref{apx:lyapunov} to highlight this idea) and (ii) utilizing the last-iterate high probability convergence of stochastic mirror descent method to analyze \CO{}. 
    %\item In addition to comparing our work to online resource allocation, we also highlighted a key deviation from the literature on dynamic matching of queues, due to the reversed order of waiting and matching (in the last two paragraphs of \Cref{subsec:lit+review}). Furthermore, we emphasized our main contribution of designing distribution-free algorithms for refugee matching (in the third paragraph of \Cref{subsec:lit+review}) as acknowledged in the meta review.
    \item We also highlighted our technical result pertaining to  the regret of our second algorithm (\Cref{ALG+Surrogate+P}) in the near-critical regime (\Cref{def:eps+regimes}) by presenting \Cref{thm:near+critical} in \Cref{subsec:alg+surrogate+primal} (rather than in the appendix) and elaborating on its implication about the fundamental benefit of accounting for the backlog in the near-critical regime in the paragraph following \Cref{thm:near+critical}. 
%\item We have added \Cref{thm:near+critical} in \Cref{subsec:alg+surrogate+primal}, which was deferred to appendix in the EC version (due to page limitation), that provides a lower bound of \CO{}'s regret under the near near-critical regime (\Cref{def:eps+regimes}). In a nutshell, \Cref{thm:near+critical} (and the related discussion) shows that while \CA{} and \CO{} are equally powerful under the stable regime (\Cref{def:eps+regimes}), \CA{} has a better regret guarantee than \CO{} under the near-critical regime and for a large value of $\BuildUpCost$ (penalty parameter for congestion), highlighting inherent benefit of the backlog information. 
\item We have also provided additional intuition on the proof ideas behind our theoretical results throughout the paper, including: (i) {the discussion following equation \eqref{eq:K_t} to explain the design of our pseudo-rewards for proving \Cref{thm:ALG+Surrogate+Dual}}; (ii) the paragraph following \Cref{lemma:pseudo+upper} to clarify how we apply classical online learning regret in our analysis; and (iii) the last paragraph of \Cref{subsec:ALG+D+pfsketch}, which elaborates on additional steps of our proof of \Cref{thm:ALG+Surrogate+Dual}.
\end{enumerate}
\end{itemize}

\begin{comment}
\item{\bf Improving Exposition.} Based on the insightful comments from the EC reviews and meta reviews, we have added significant clarifications and elaborations in various sections to further elaborate our modeling choices and highlight our technical contributions. In particular, our changes include the following.
\begin{enumerate}[label=
    (\alph*)]
    \item {\bf Elaboration on modeling choices.} 
    \item {\bf Highlighting Technical Aspects}
    \begin{enumerate}[label=
    (\roman*)]
    \item In response to Reviwer B's comment, taking into account that we provided a short version of literature review in the conference version of the paper (due to space limitation), we have significantly expanded the literature review in \Cref{subsec:lit+review} to better highlight our technical contribution. Specifically, in the seventh paragraph of \Cref{subsec:lit+review}, we emphasized that, while we draw on classical scoring techniques in online resource allocation, the time-varying nature of dual variables (\Cref{prop:offline}) deviates from the literature. Consequently, we introduce several innovative ideas including (i) novel combination of adversarial learning and drift analysis to design and analyze \CA{} (we have also added \Cref{apx:lyapunov} to highlight this idea) and (ii) utilizing the last-iterate high probability convergence of stochastic mirror descent method to analyze \CO{}. 
\item In addition to comparing our work to online resource allocation, we also highlighted a key deviation from the literature on dynamic matching of queues, due to the reversed order of waiting and matching (in the last two paragraphs of \Cref{subsec:lit+review}). Furthermore, we emphasized our main contribution of designing distribution-free algorithms for refugee matching (in the third paragraph of \Cref{subsec:lit+review}) as acknowledged by the meta review.
\item We have added \Cref{thm:near+critical} in \Cref{subsec:alg+surrogate+primal}, which was deferred to appendix in the conference version due to page limitation, that compares the theoretical performance of \CA{} and \CO{} in the near-critical regime (\Cref{def:eps+regimes}). In particular, our result shows that while both algorithms are equally powerful in the stable regime (\Cref{def:eps+regimes}), \CA{} has a better regret guarantee than \CO{} in the near-critical regime, highlighting inherent benefit of the backlog information. 
\item In response to Reviewer A's comment, we have added several sentences to provide additional intuition on the proof ideas behind our theoretical results, including: (i) \SLedit{the paragraph following equation \eqref{eq:K_t} to explain the design of our pseudo-rewards for proving \Cref{thm:ALG+Surrogate+Dual}}; (ii) the last sentence in the paragraph following \Cref{lemma:pseudo+upper} to clarify how we apply classical online learning regret in our analysis; and (iii) the last paragraph of \Cref{subsec:ALG+D+pfsketch}, which elaborates additional steps to conclude our proof.
\end{enumerate}
\end{enumerate}
%%%%%%%%%%%%%%%%%%%%%%%%%%%%%%%5

\end{comment}


\begin{comment}
\SLcomment{Old version below}
\begin{itemize}
% Part 1: 
    \item {\bf Expanding Models and Algorithms.} In this version, we have added two sections extend our model and algorithms to incorporate additional aspects related to refugee resettlement. In particular,
\begin{enumerate}[label=(\alph*)]
    \item In response to EC Review 2 and Meta reviews, in  \Cref{apx+non+unit+size}, we present how our model and algorithms can incorporate multiple knapsack constraints.
    \item In response to EC Review 3, in \Cref{apx+batching}, we provide a simple adpatation of our algorithm to incorporate batched arrivals. Through the numerical case study, we demonstrate that the heuristic can achieve a mild performance improvement compared to the fully online version of our algorithm. \ECcomment{Please feel free to take a pass at \Cref{apx+batching} too. Please also note that I added a few sentences (colored green) in \Cref{sec:numerics} to refer to these new appendix sections}
\end{enumerate}
%%%%%%%%%%%%%%%%%%%%%%%%%%%%%%%%%%%%
\item {\bf Highlighting Technical Aspects.} Following the suggestions made in the meta review and EC reviews, we have added substantial elaborations in the main body to  highlight our technical contributions. In particular, 
\begin{enumerate}[label=(\alph*)]
\item Taking into account that we provided a short version of literature review in the conference version of the paper (due to space limitation), we have significantly expanded the literature review in \Cref{subsec:lit+review} to better highlight our technical contribution. Specifically, we emphasized that, while we draw on classical scoring techniques in online resource allocation, the time-varying nature of dual variables (\Cref{prop:offline}) deviates from the literature. Consequently, we introduce innovative ideas including (i) novel combination of adversarial learning and drift analysis to design and analyze \CA{} (we have also added \Cref{apx:lyapunov} to highlight this idea) and (ii) utilizing the last-iterate high probability convergence of stochastic mirror descent method to analyze. 
\item Beside the comparison to online resource allocation, we further highlighted in \Cref{subsec:lit+review} (i) a fundamental deviation from literature on dynamic matching of queues due to the reversed order of waiting and matching, and (ii) our main contribution of designing the distribution-free algorithms to literature on refugee matching, as acknowledged by the meta review.
\item We have added \Cref{thm:near+critical} in \Cref{subsec:alg+surrogate+primal}, which was deferred to appendix in the conference version due to page limitation, that compares the theoretical performance of \CA{} and \CO{} in the near-critical regime (\Cref{def:eps+regimes}). In particular, our result shows that while both algorithms are equally powerful in the stable regime (\Cref{def:eps+regimes}), \CA{} has a better regret guarantee than \CO{} in the near-critical regime, highlighting inherent benefit of the backlog information. 

%EC Review 2: highlighting ``new'' ideas --- lit review significantly expanded (due to space limitation the original version was super short) where we highlight  a fundamental difference from (i) online resource allocation (and in particular the classic scoring techniques) due to the time-varying duals (ii) queueing literature to the reversed order of waiting and matching. These differences require developing new technical ideas, including (i) a novel combination of the Lyapunov theory and adversarial online learning for CA-DL (ii) last-iterate high-probability convergence of the stochastic mirror descent methods for CO-DL. \SLcomment{\bf Maybe \@Rad can help me this..}
%\item New Appendix on alternative interpretation of our algorithm building on Lyanpuov theory? \SLcomment{would this be the right place of this item?}
\end{enumerate}


    % enumerate end
%%%%%%%%%%%%%%%%%%%%%%%%%%%%%%%%%%%%%%%%%%%%%%%%%%%%%%%%%
% Part 2:
\item {\bf Improving Expositions.} 
Based on the insightful comments from the EC reviews and meta reviews, we have added significant clarifications and elaborations throughout the paper. In particular, 
    \begin{enumerate}[label=(\alph*)]
    \item In response to EC Review 1, we have added elaborations throughout \Cref{sec:intro} on the motivation for distribution-free algorithms for our partner agency. Specifically, in \Cref{subsec:intro+background}, we clarified that (i) the decision-making horizon for refugee resettlement is one year, and (ii) Figure \ref{fig:tied+proportion} suggests that data from past years is an unreliable source of ``distributional knowledge" for future arrivals, hence motivating us to develop distribution-free algorithms. Finally, we clarified that we assume the arrival sequence \emph{within the year} follows an unknown i.i.d. distribution (which may differ from year to year, as evidenced in \Cref{fig:tied+proportion}) for technical analysis. \ECedit{Additionally, we have added \Cref{apx+within+year+variations} to provide further numerical evidence supporting the within-year stationarity assumption.}\ECcomment{I added this appendix. It would be great if you can take a pass. Please also note that I added a sentence in \Cref{sec:numerics} (in green color) to refer to this appendix. }
    \item Based on comments made by EC review 1, we added significant clarifications and elaborations in the technical part of the paper (Section \ref{sec:model}-\ref{subsec:alg+surrogate+primal}), including (i) a paragraph after \Cref{def:eps+regimes} to clarify our motivation for defining the two separate regimes (namely, stable and near-critical) regarding the service slack parameter $\ServiceSlack$ (ii) more intuitions throughout the proof sketches in the main body (\Cref{subsec:ALG+D+pfsketch}, for example). 
    \item In response to EC review 3, in \Cref{subsec:intro+background}, we have further highlighted the importance of post-allocation service for our partner agency, noting that the current practice is mainly driven by load-balancing without a systematic attempt to optimize employment outcomes. We also highlight that the post-allocation service is not misaligned with respecting the target annual quota because our soft and hard constraints for static resources incorporate the agency's desire to respect the annual quota.
    %EC Review 3: Importance of post-allocation service
    %\item We have added many other clarifications and elaborations, including (i) a more explicit statement that (i) \ECedit{more intuitive expositions regarding the proof sketches in the main body,} .   
\end{enumerate}
% Part 3
%%%%%%%%%%%%%%%%%%%%%%%%%%%%%%%%%%%%%%%%%%%%%%%%%%%%%%%%%
\end{itemize}
    
\end{comment}
